# Supplementary material for: Design Considerations for Factorial Adaptive Multi-Arm Multi-Stage (FAST) Clinical Trials
Source: arXiv:2310.12830 source file (2023-10-19)

# Appendix A: Graphs

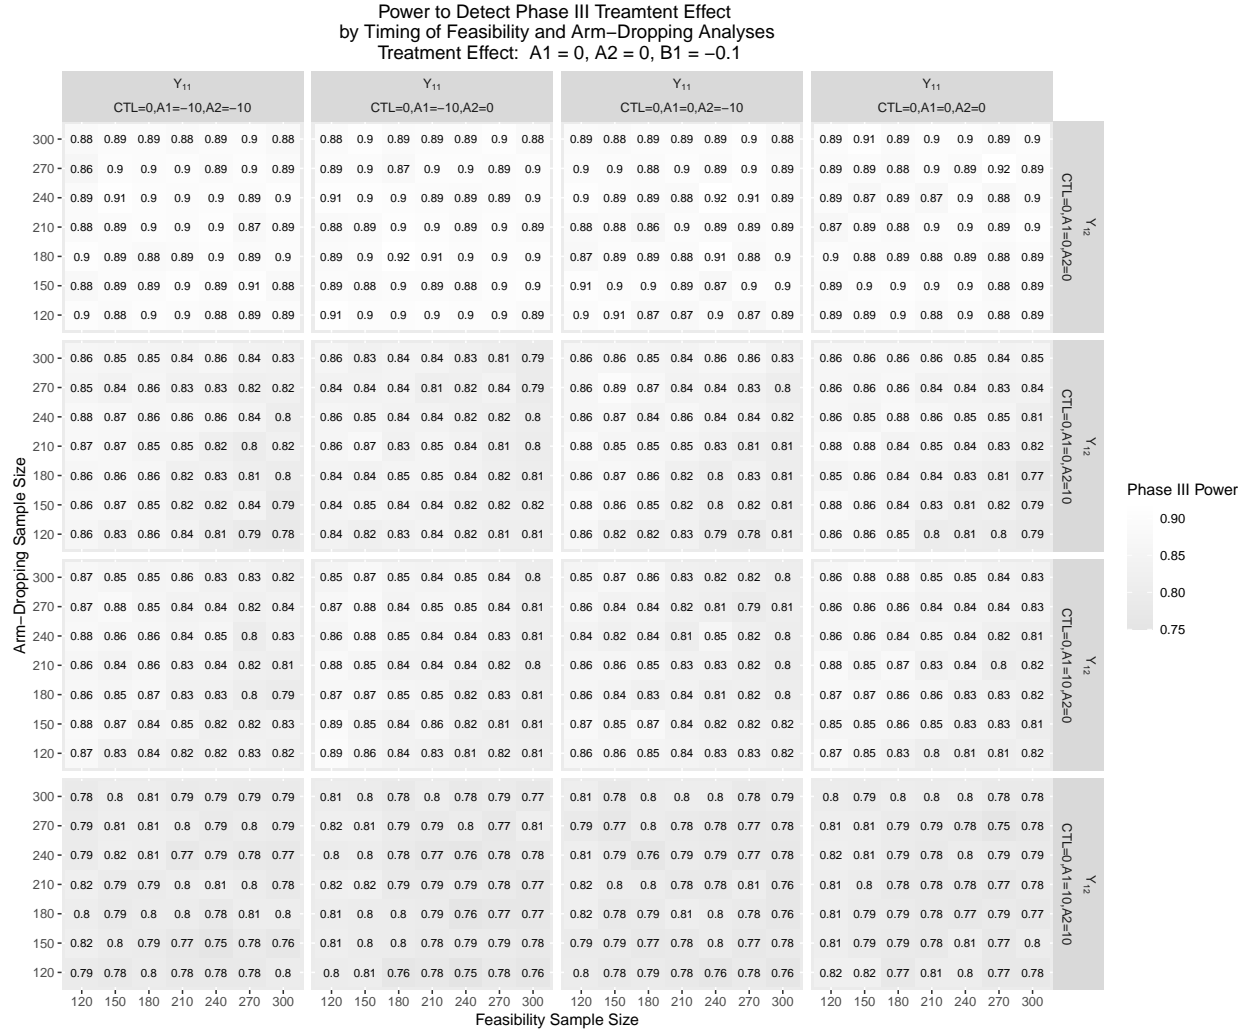

Power to Detect Phase III Treatment Effect  
by Timing of Feasibility and Arm-Dropping Analyses  
Treatment Effect:  $A1 = 0, A2 = 0, B1 = 0$

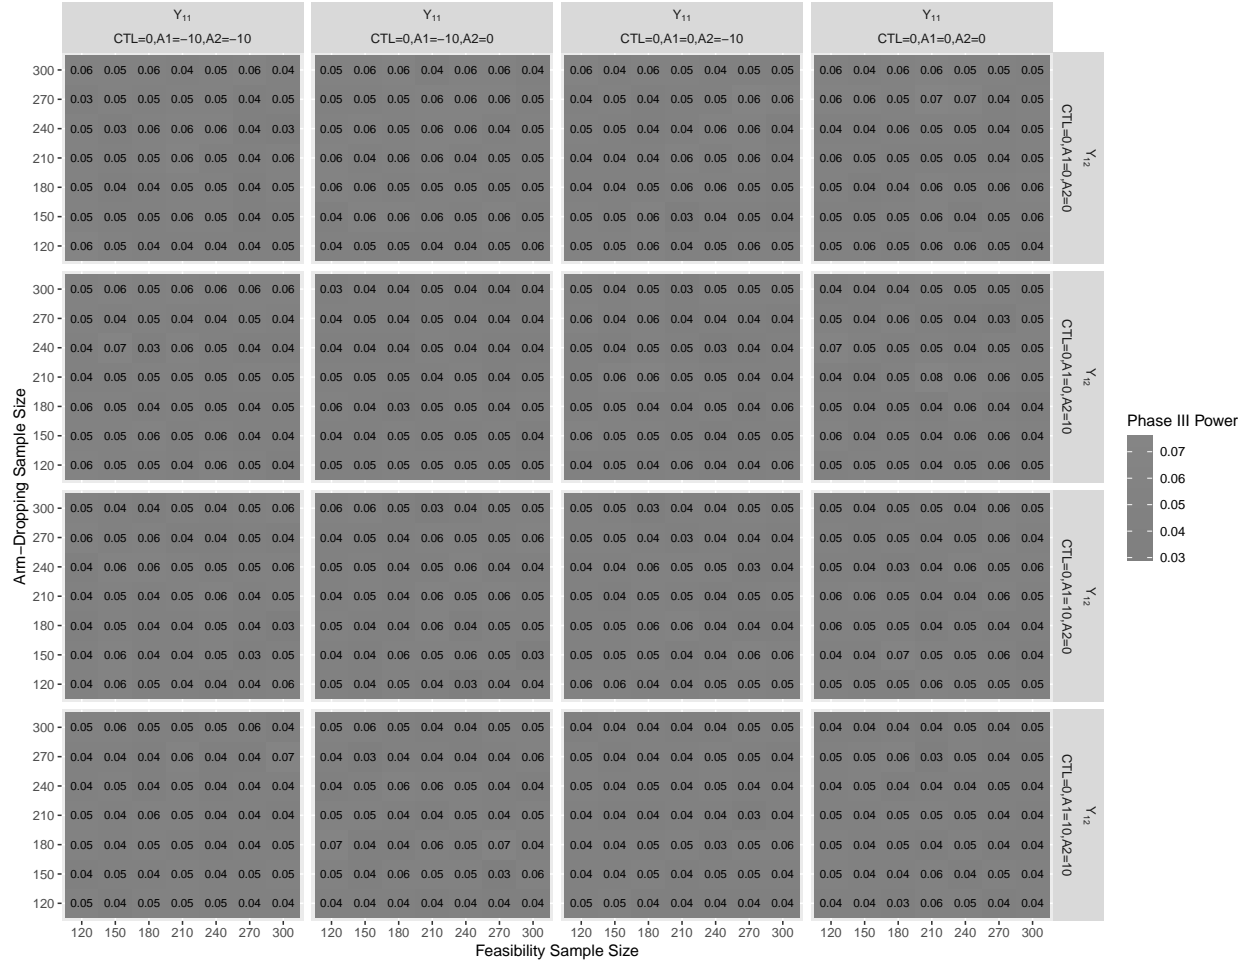

Power to Detect Phase III Treatment Effect  
by Timing of Feasibility and Arm-Dropping Analyses  
Treatment Effect:  $A1 = 0$ ,  $A2 = 0.1$ ,  $B1 = -0.1$

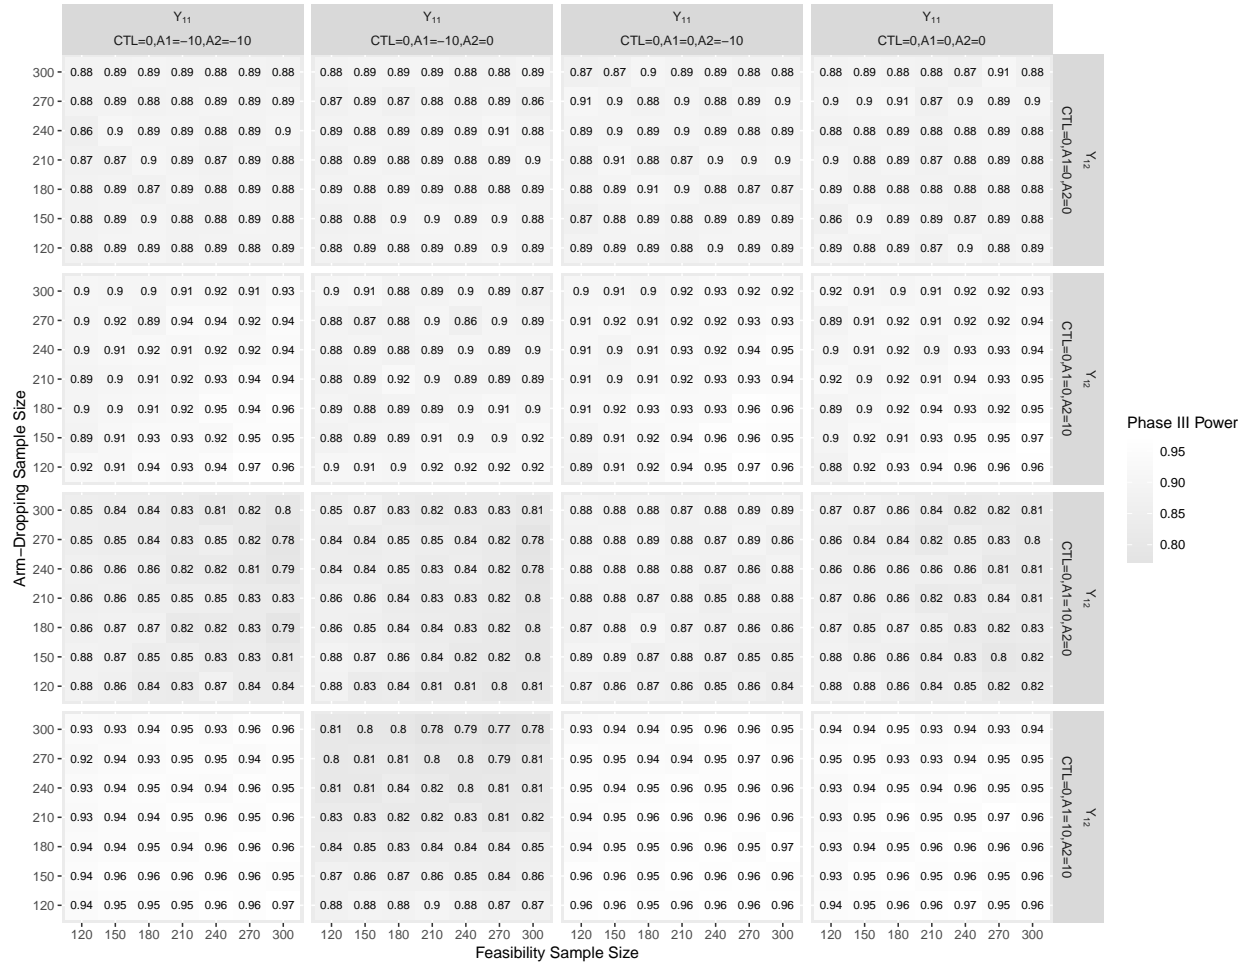

Power to Detect Phase III Treatment Effect  
by Timing of Feasibility and Arm-Dropping Analyses  
Treatment Effect:  $A1 = 0, A2 = 0.1, B1 = 0$

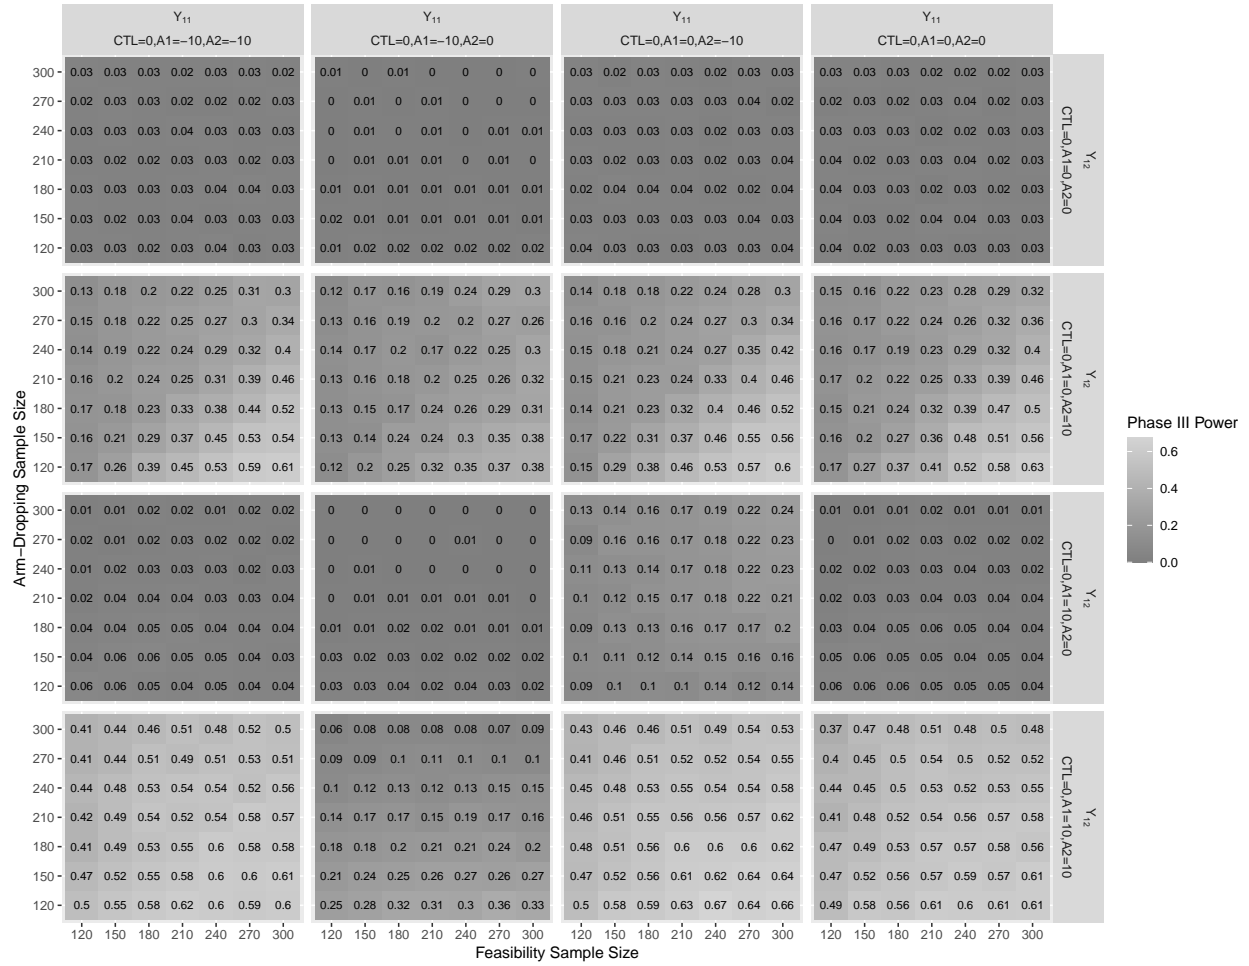

Power to Detect Phase III Treatment Effect  
by Timing of Feasibility and Arm-Dropping Analyses  
Treatment Effect:  $A1 = 0.1$ ,  $A2 = 0$ ,  $B1 = -0.1$

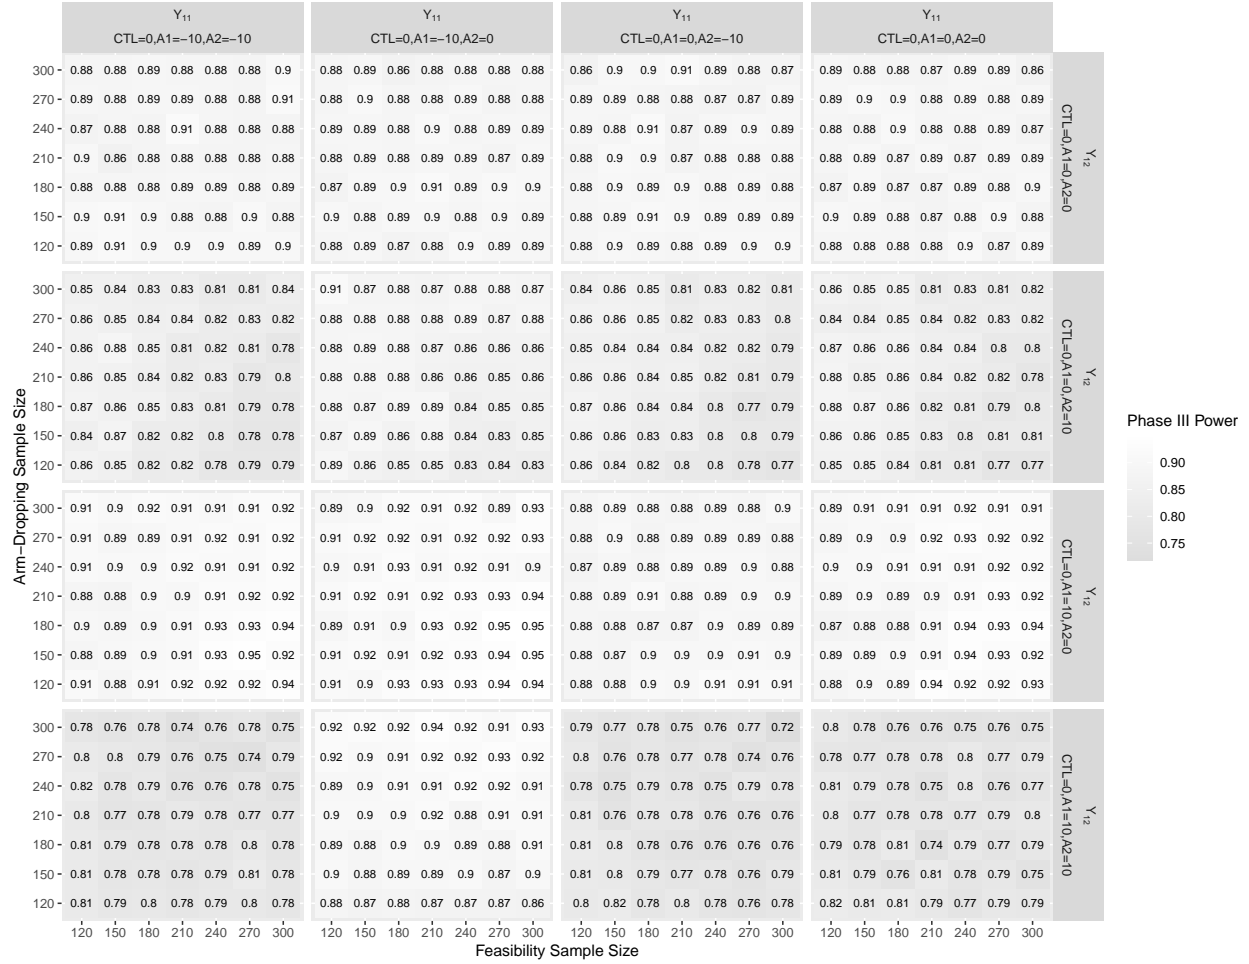

Power to Detect Phase III Treatment Effect  
by Timing of Feasibility and Arm-Dropping Analyses  
Treatment Effect:  $A1 = 0.1$ ,  $A2 = 0$ ,  $B1 = 0$

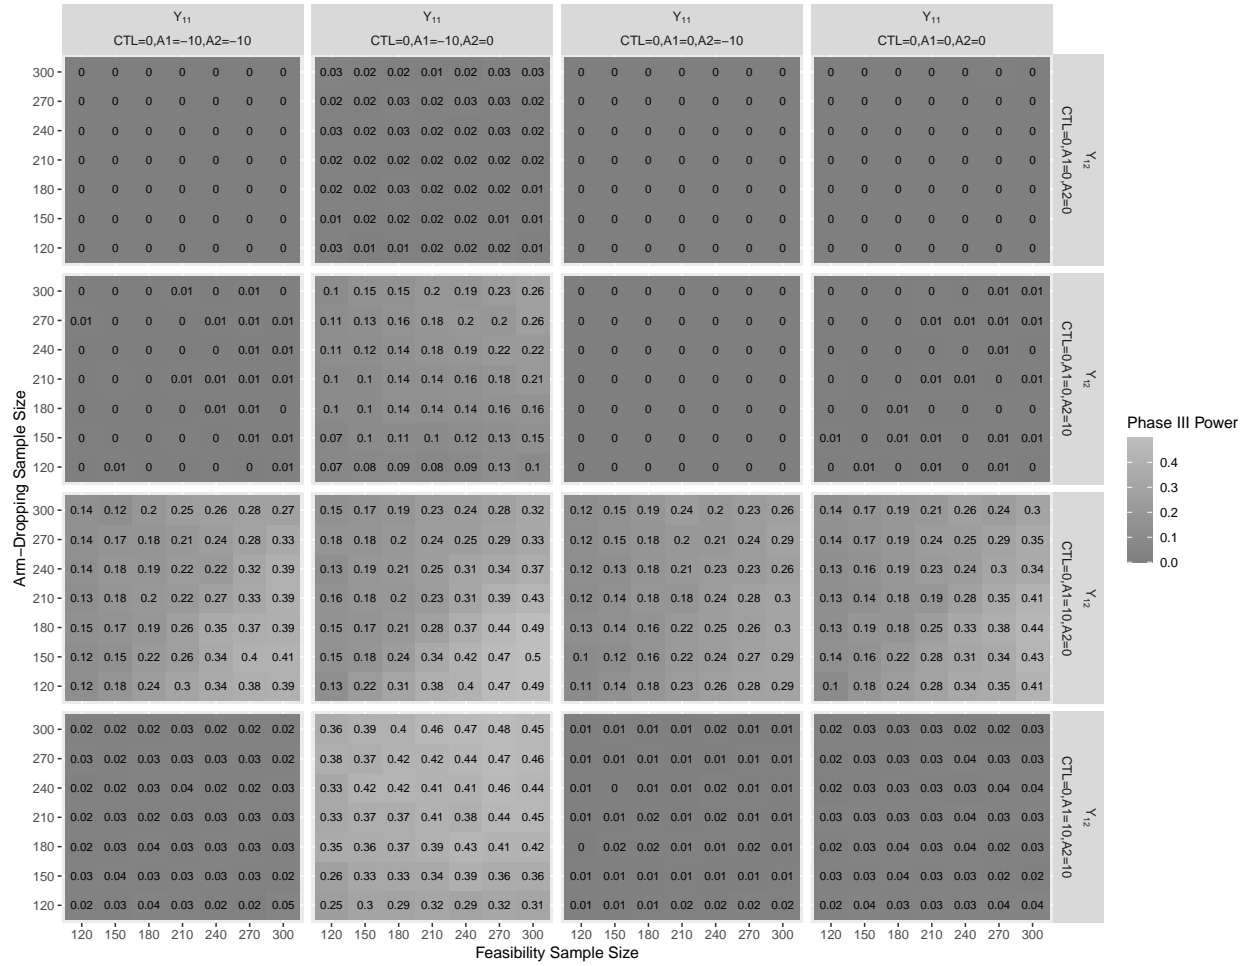

Power to Detect Phase III Treatment Effect  
by Timing of Feasibility and Arm-Dropping Analyses  
Treatment Effect:  $A1 = 0.1, A2 = 0.1, B1 = -0.1$

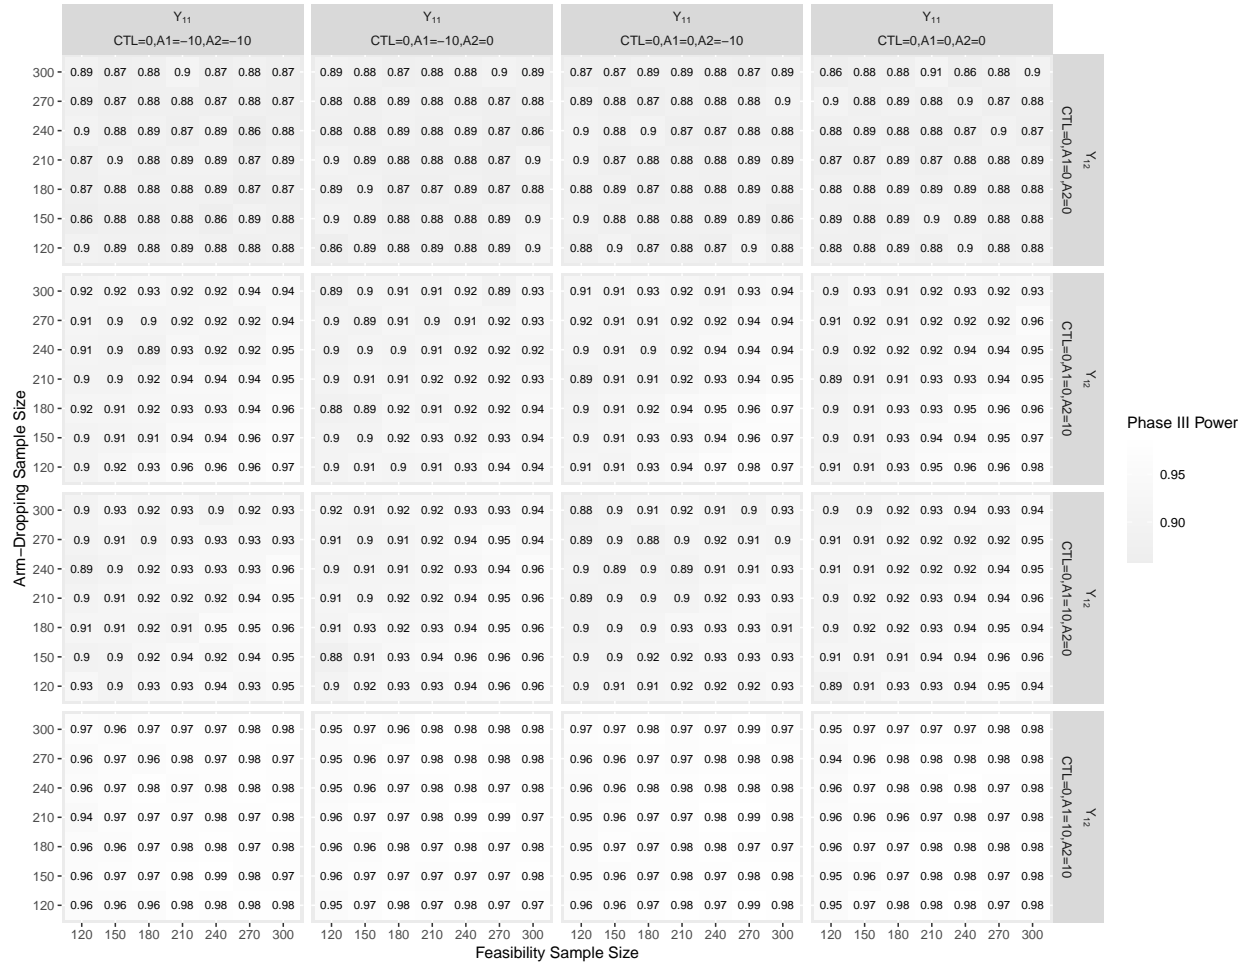

Power to Detect Phase III Treatment Effect  
by Timing of Feasibility and Arm-Dropping Analyses  
Treatment Effect:  $A1 = 0.1, A2 = 0.1, B1 = 0$

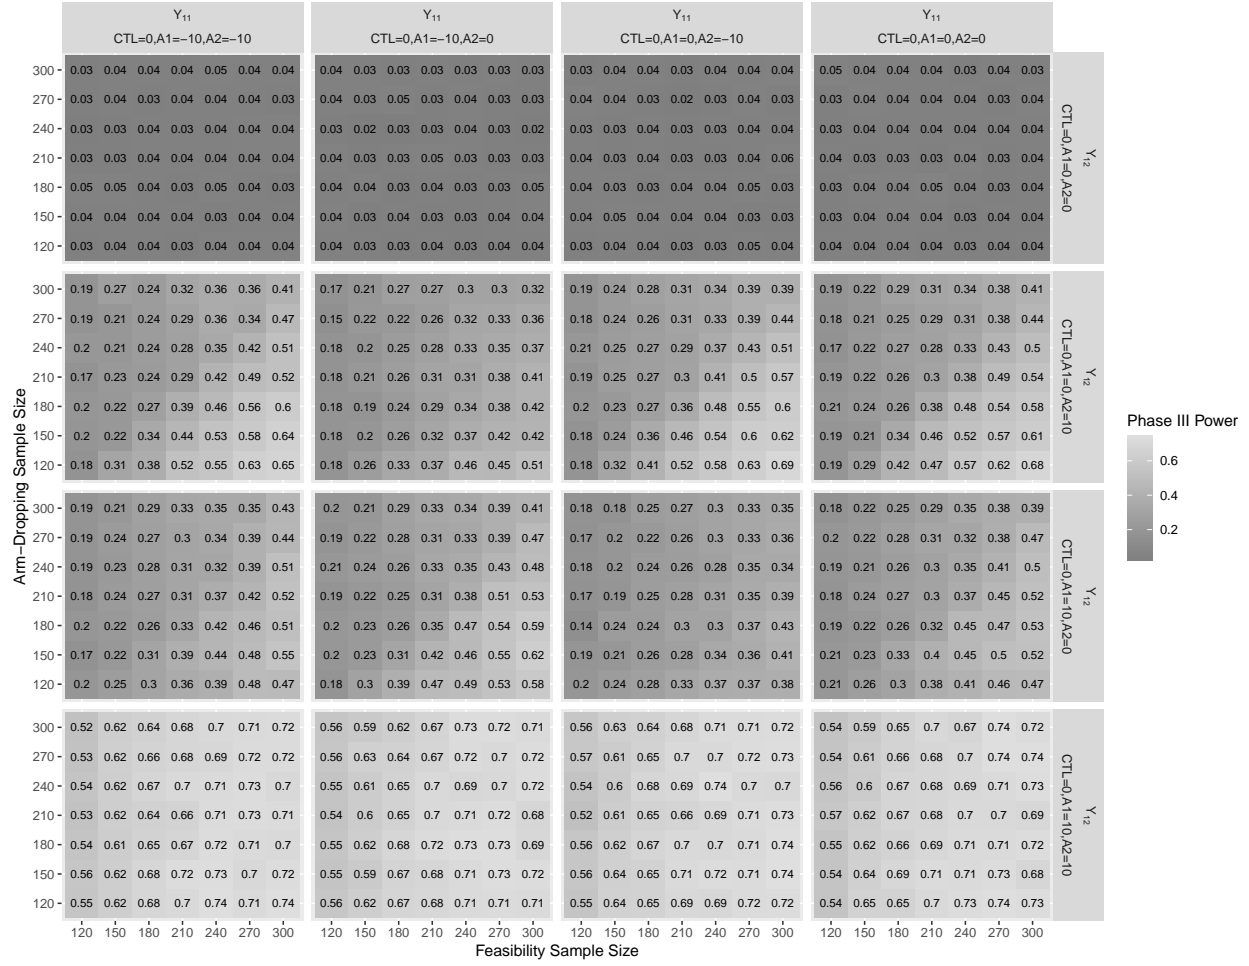

Probability of Correct Decision during Arm-Dropping Analysis  
by Timing of Feasibility and Arm-Dropping Analyses  
Treatment Effect:  $A1 = 0, A2 = 0, B1 = -0.1$

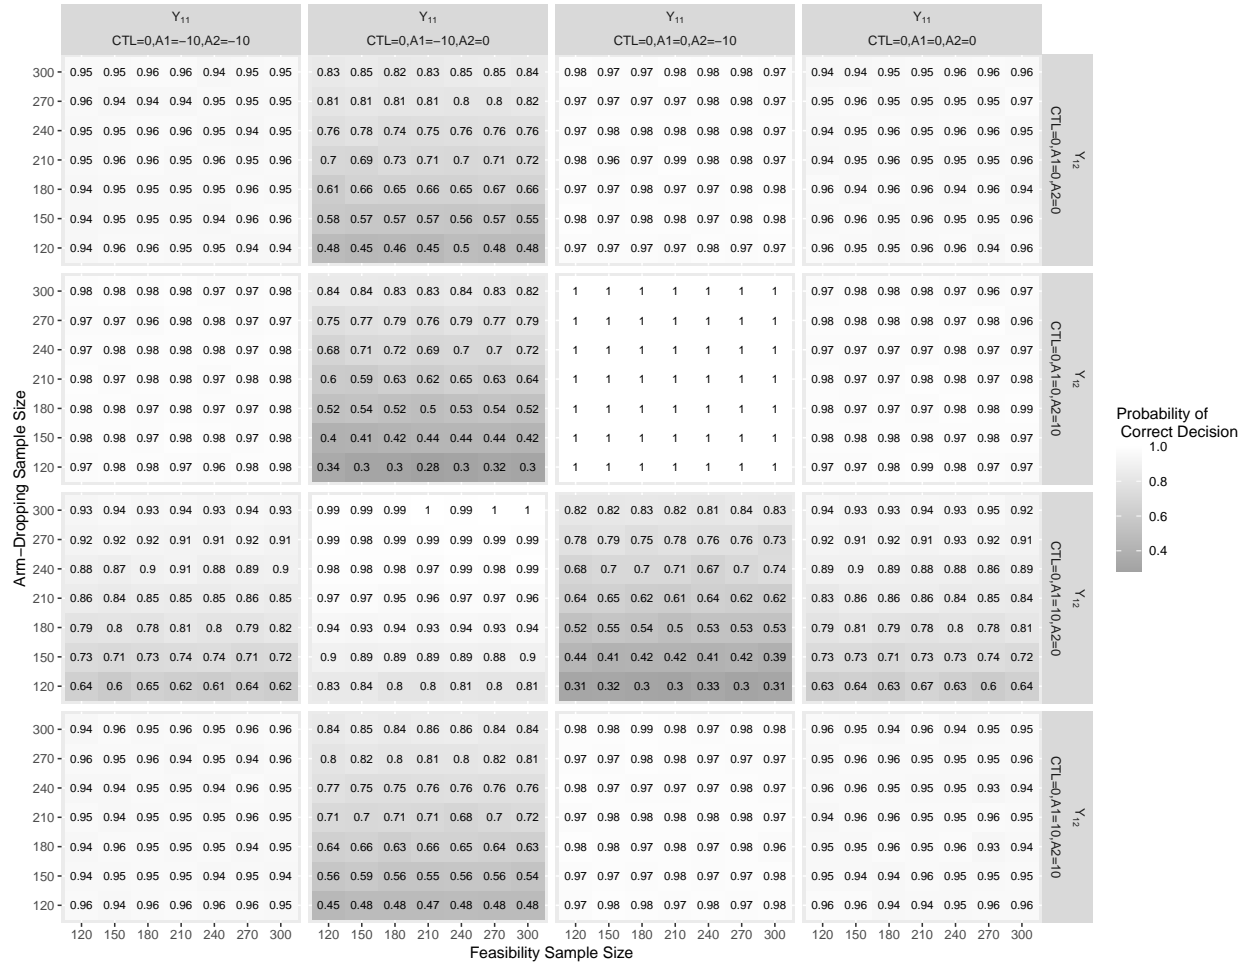

Probability of Correct Decision during Arm-Dropping Analysis  
by Timing of Feasibility and Arm-Dropping Analyses  
Treatment Effect:  $A1 = 0, A2 = 0, B1 = 0$

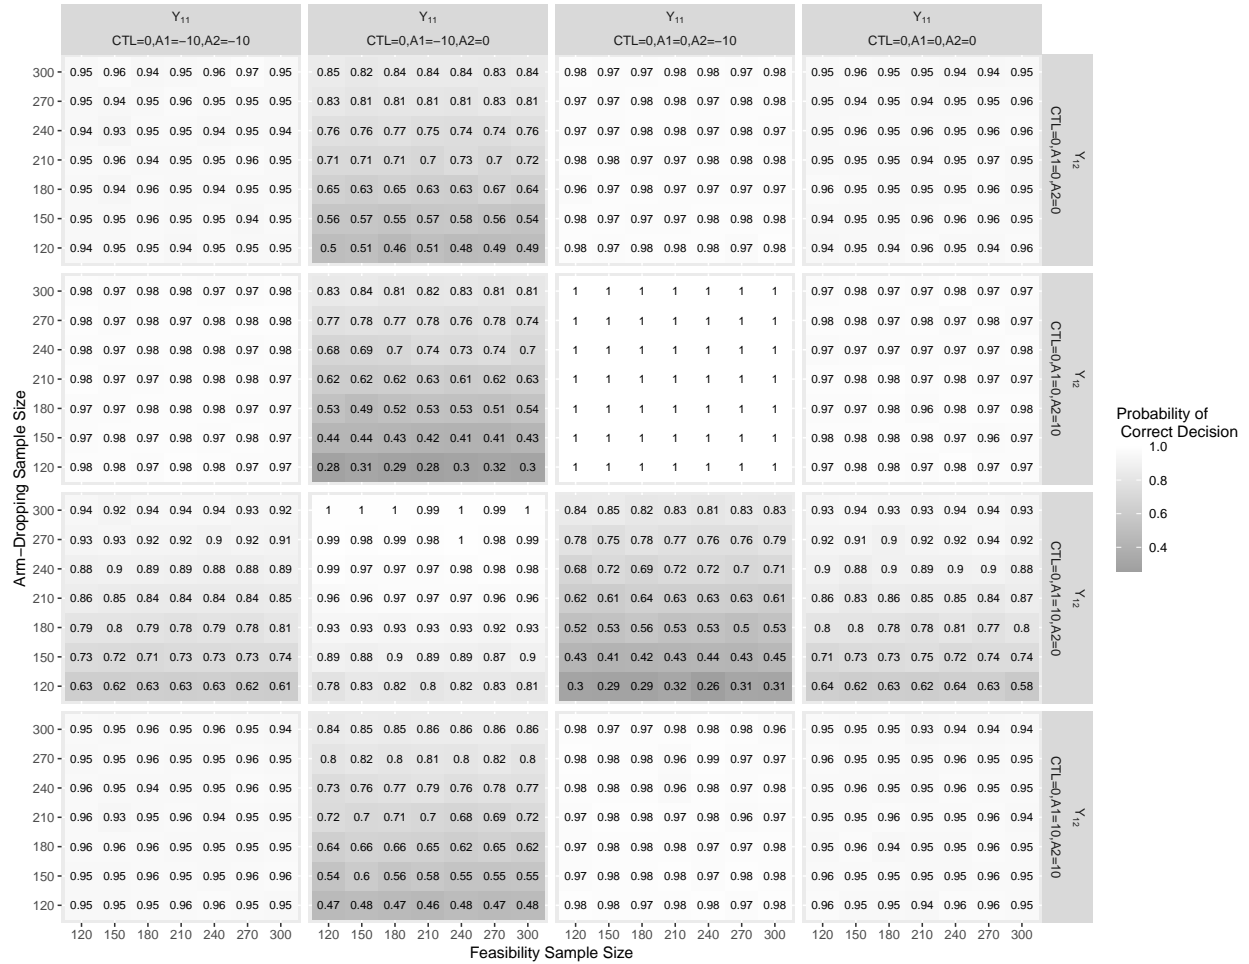

Probability of Correct Decision during Arm-Dropping Analysis  
by Timing of Feasibility and Arm-Dropping Analyses  
Treatment Effect:  $A1 = 0, A2 = 0.1, B1 = -0.1$

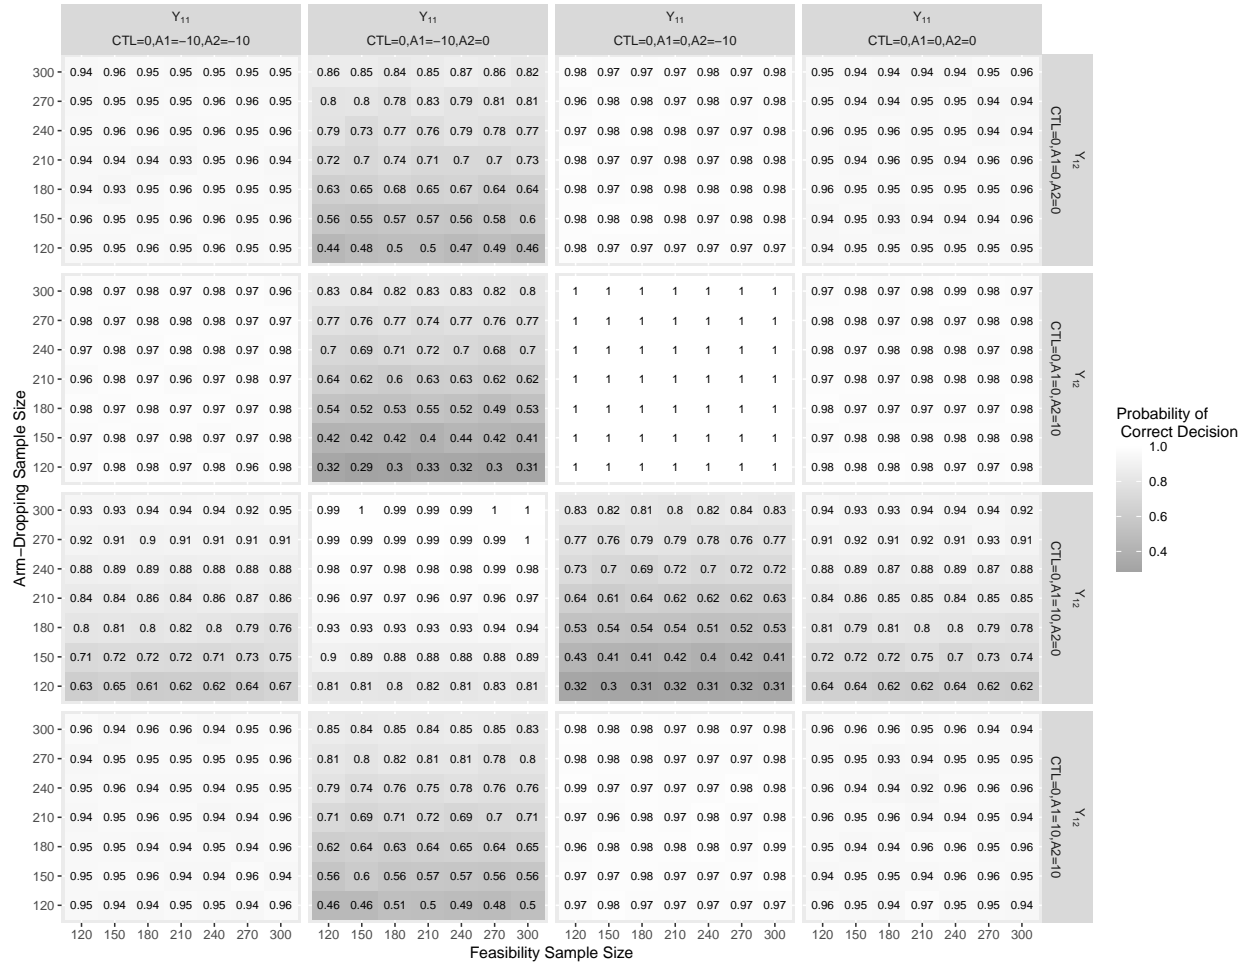

Probability of Correct Decision during Arm-Dropping Analysis  
by Timing of Feasibility and Arm-Dropping Analyses  
Treatment Effect:  $A1 = 0, A2 = 0.1, B1 = 0$

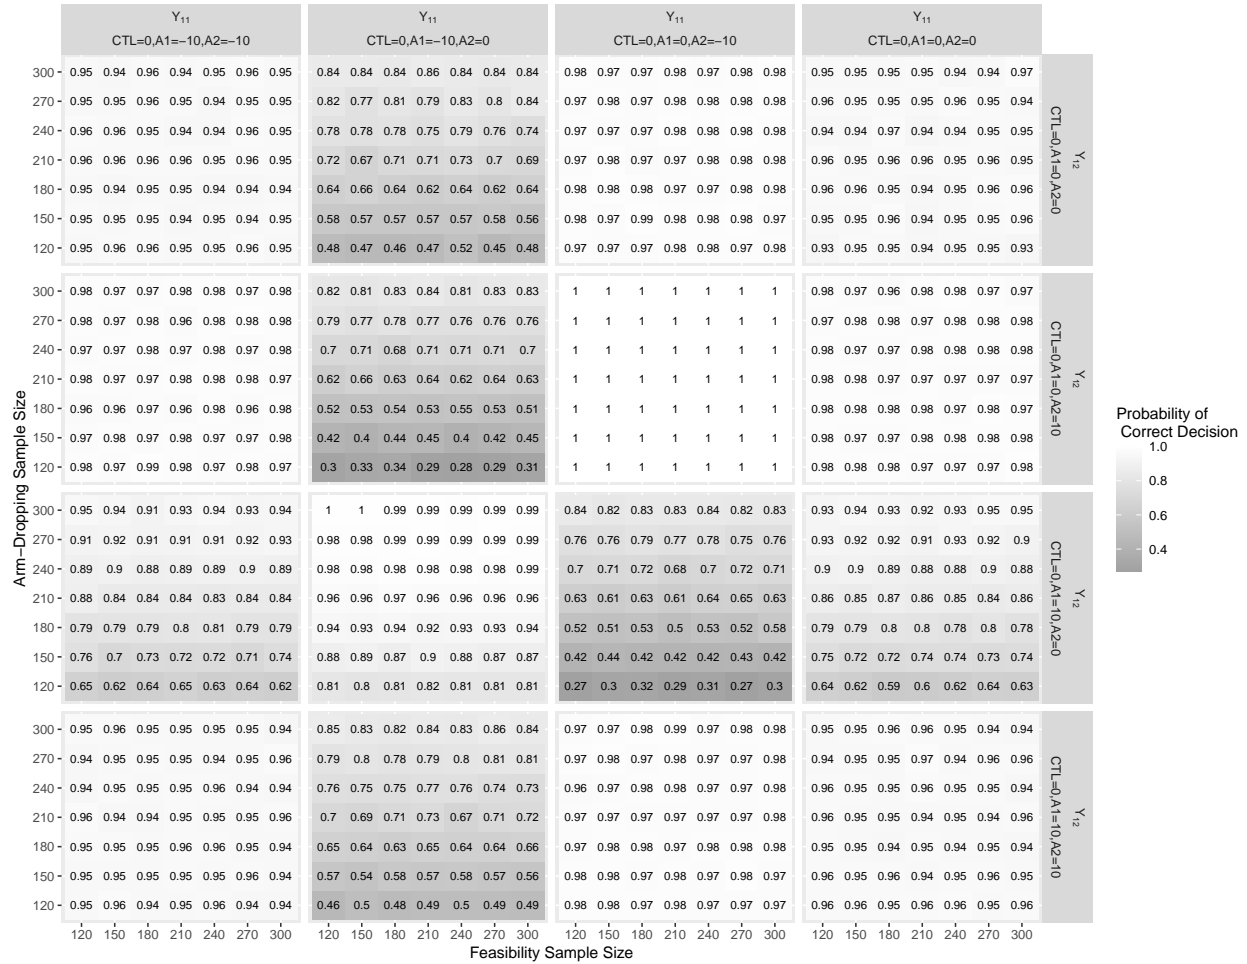

Probability of Correct Decision during Arm-Dropping Analysis  
by Timing of Feasibility and Arm-Dropping Analyses  
Treatment Effect:  $A1 = 0.1, A2 = 0, B1 = -0.1$

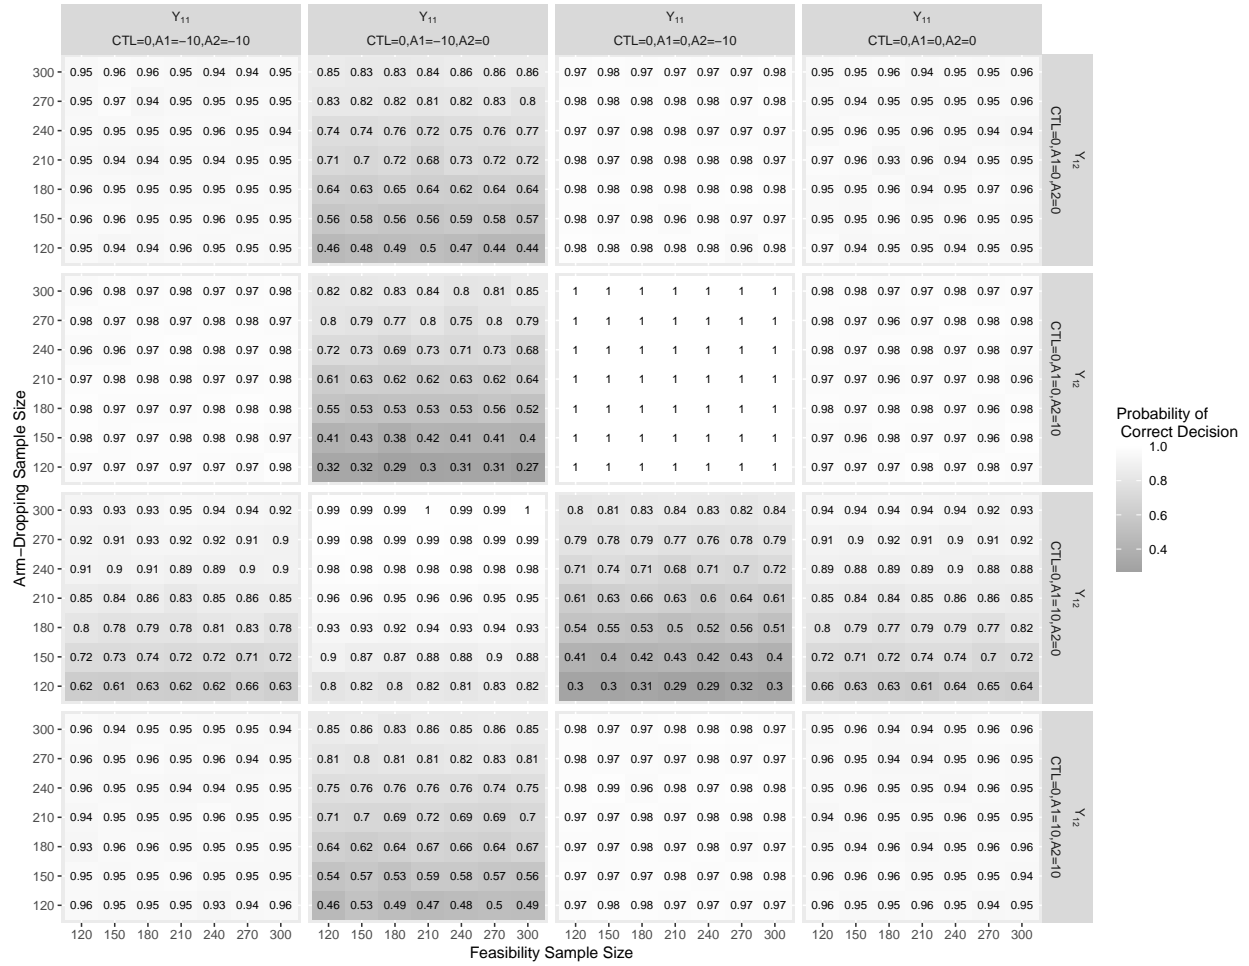

Probability of Correct Decision during Arm-Dropping Analysis  
by Timing of Feasibility and Arm-Dropping Analyses  
Treatment Effect:  $A1 = 0.1, A2 = 0, B1 = 0$

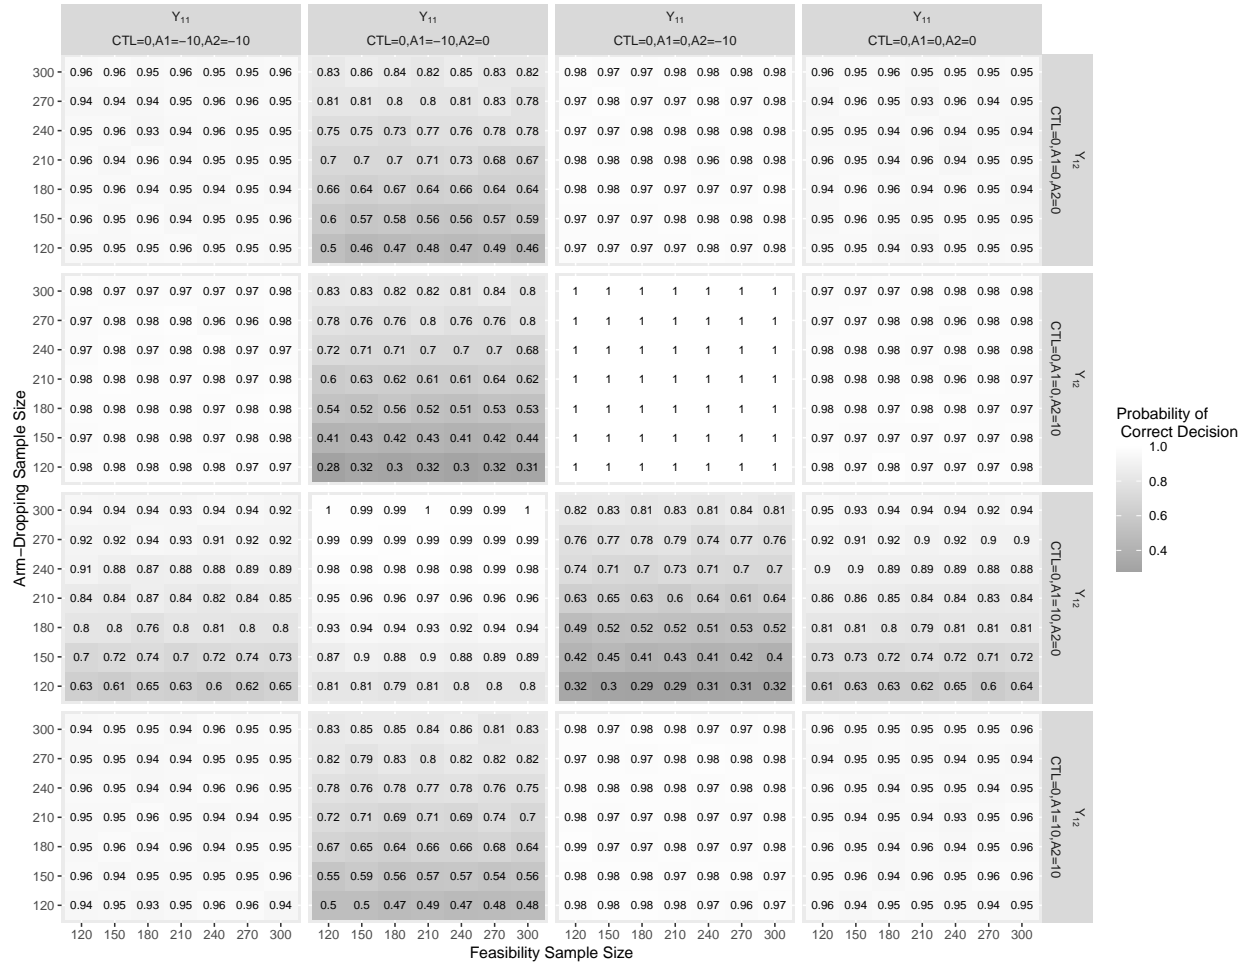

Probability of Correct Decision during Arm-Dropping Analysis  
by Timing of Feasibility and Arm-Dropping Analyses  
Treatment Effect:  $A1 = 0.1, A2 = 0.1, B1 = -0.1$

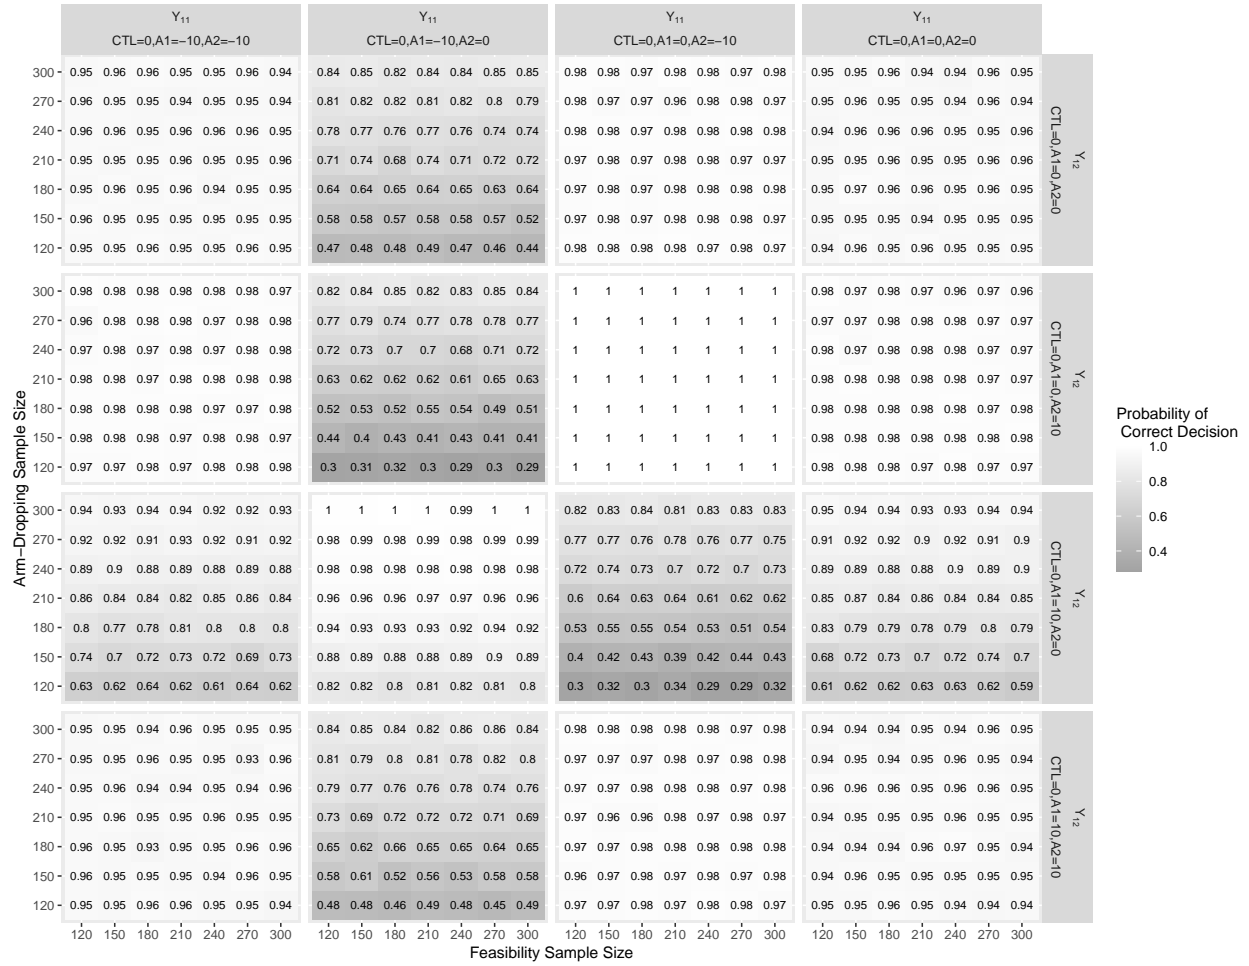

Probability of Correct Decision during Arm-Dropping Analysis  
by Timing of Feasibility and Arm-Dropping Analyses  
Treatment Effect:  $A1 = 0.1, A2 = 0.1, B1 = 0$

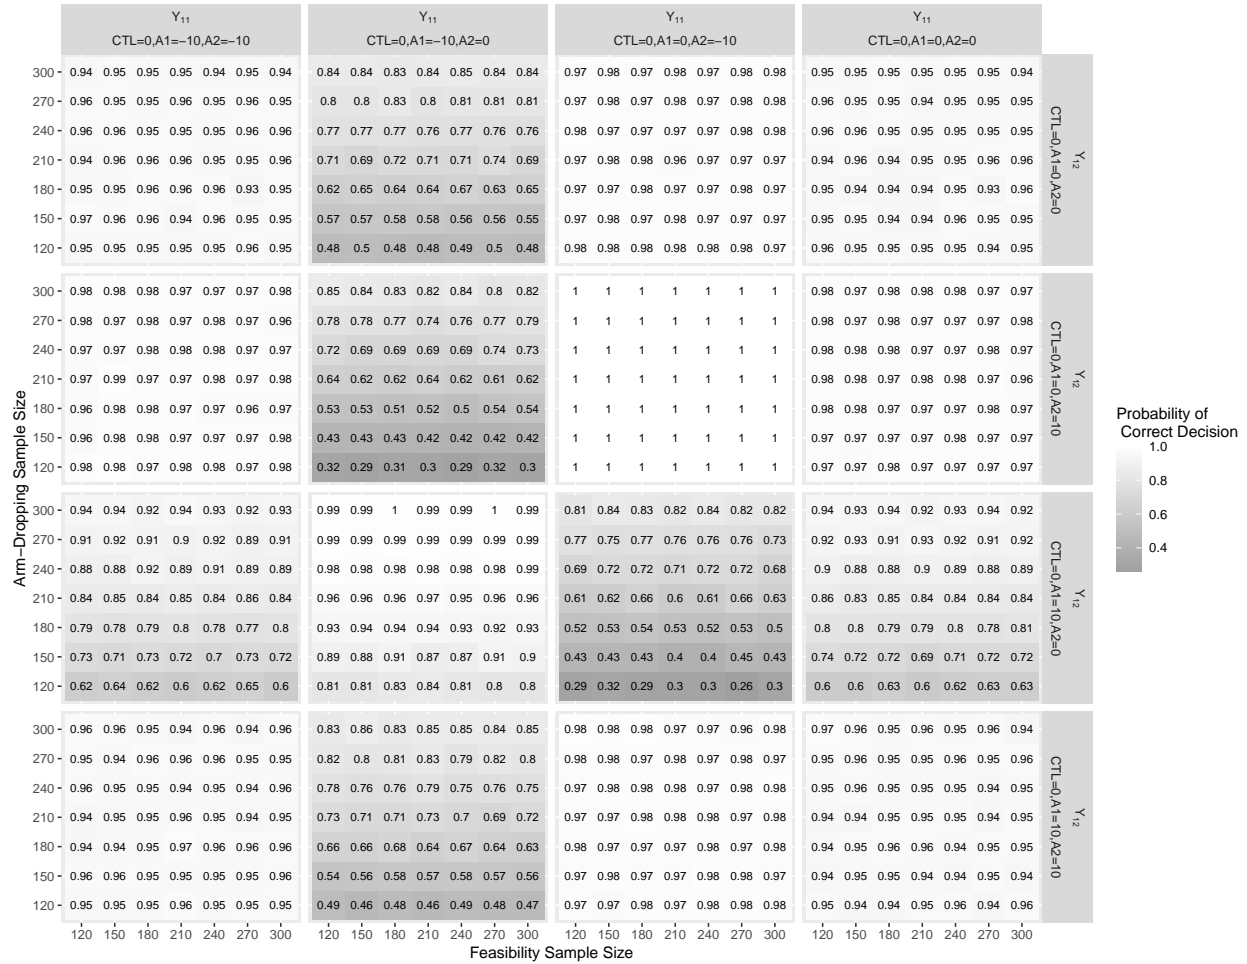

Probability Passing Feasibility Assessment  
by Timing of Feasibility and Arm-Dropping Analyses  
Treatment Effect:  $A1 = 0, A2 = 0, B1 = -0.1$

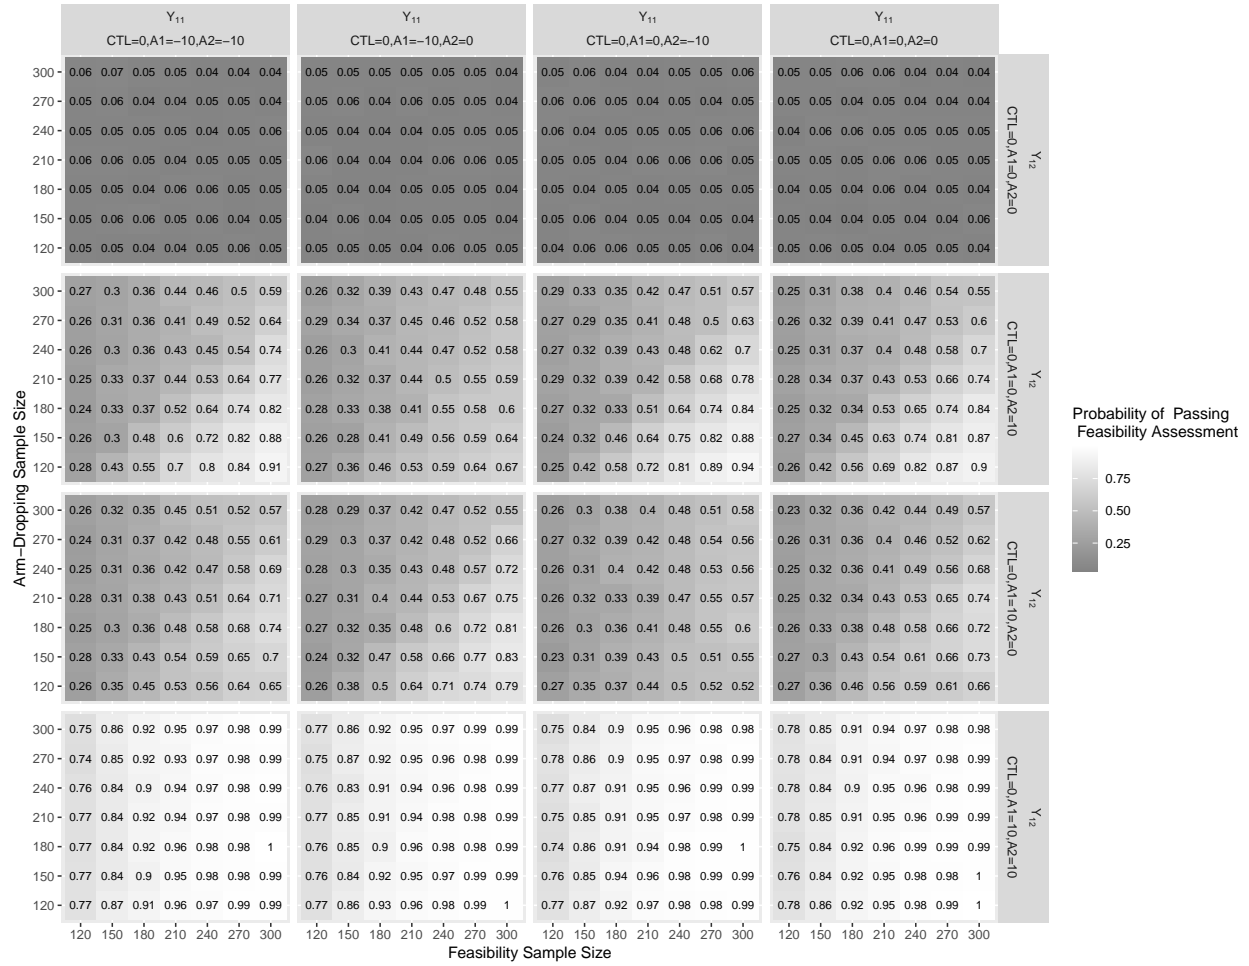

Probability Passing Feasibility Assessment  
by Timing of Feasibility and Arm-Dropping Analyses  
Treatment Effect:  $A1 = 0, A2 = 0, B1 = 0$

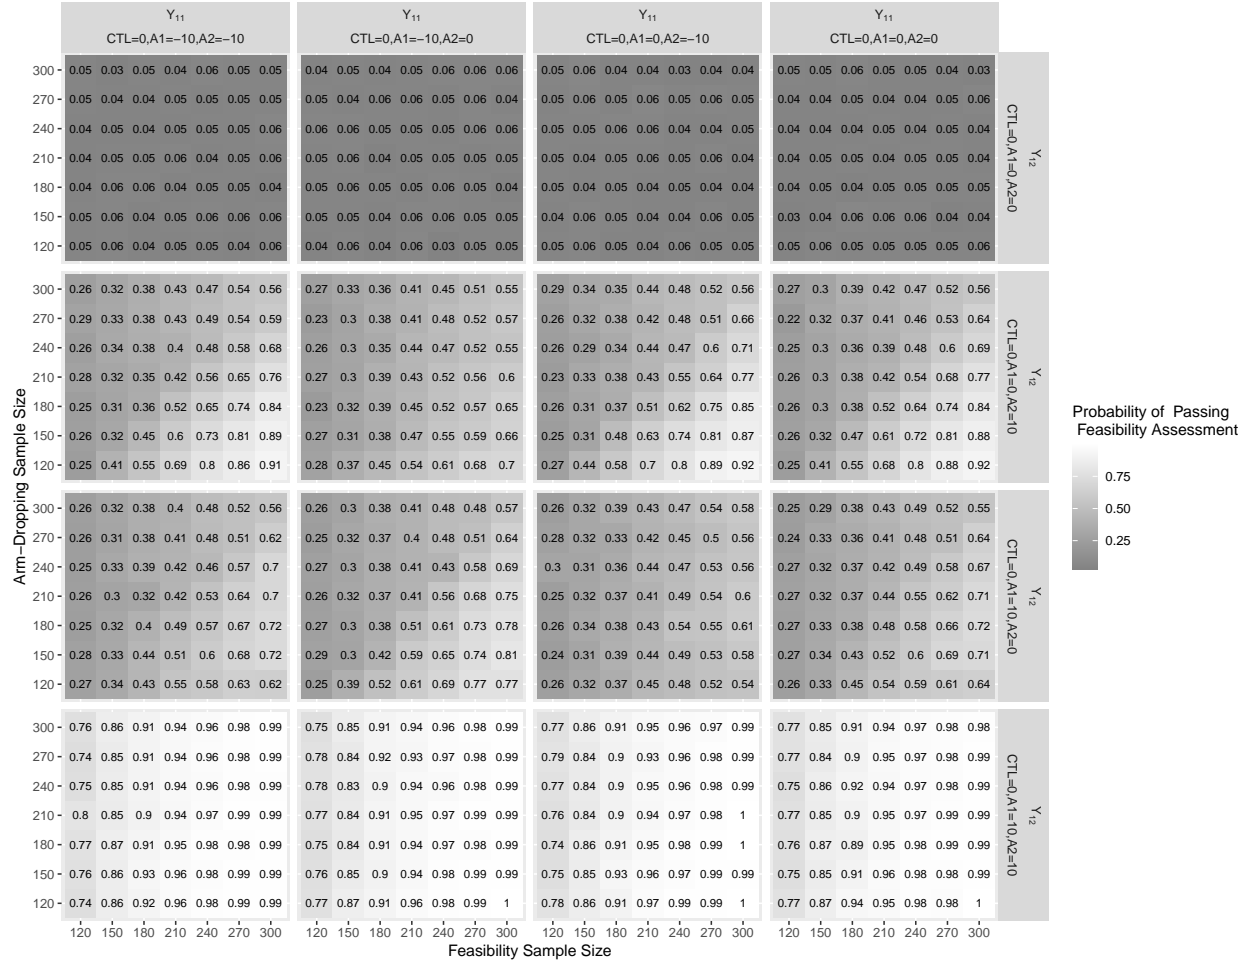

Probability Passing Feasibility Assessment  
by Timing of Feasibility and Arm-Dropping Analyses  
Treatment Effect:  $A1 = 0, A2 = 0.1, B1 = -0.1$

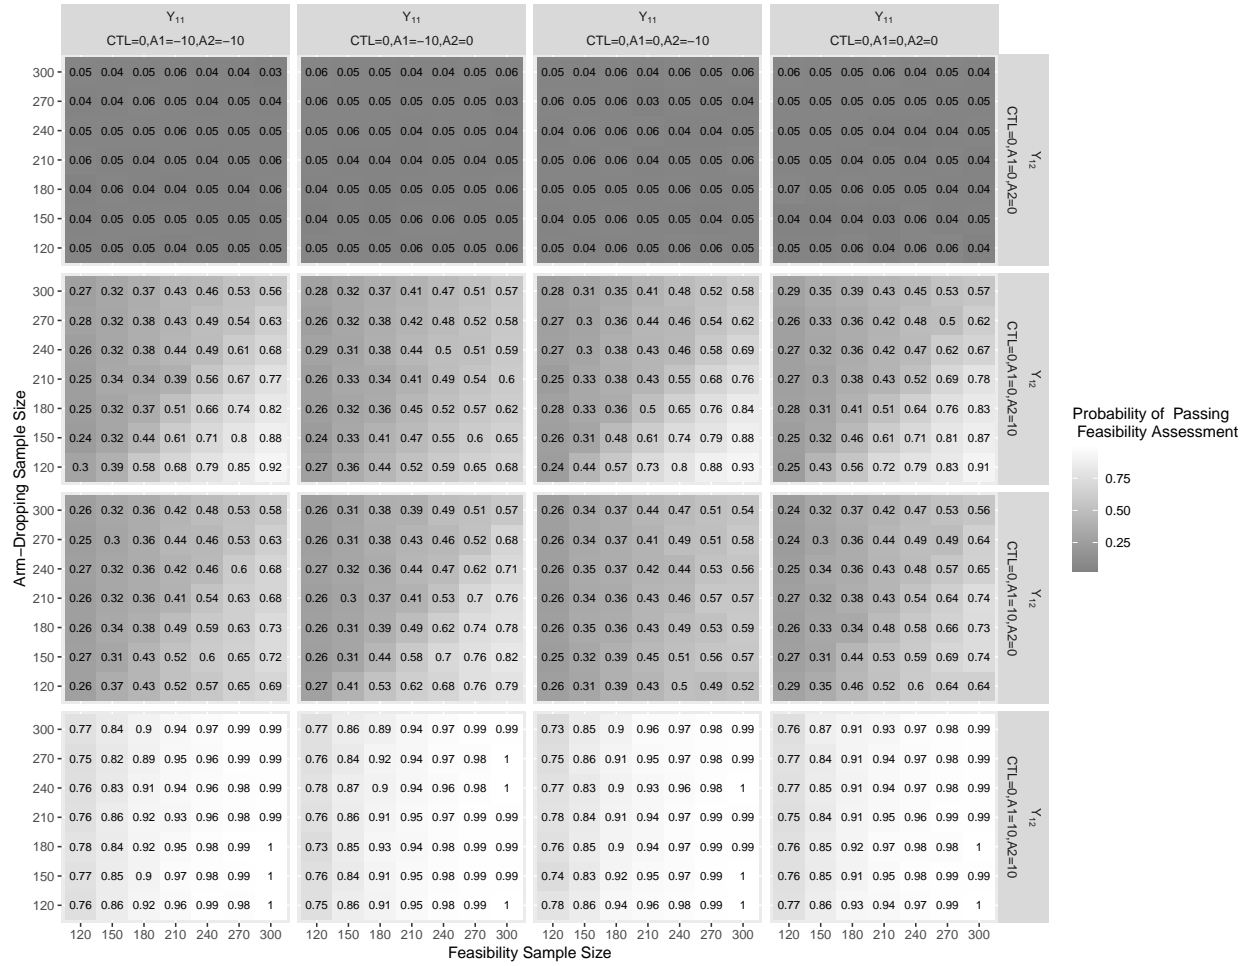

Probability Passing Feasibility Assessment  
by Timing of Feasibility and Arm-Dropping Analyses  
Treatment Effect:  $A1 = 0, A2 = 0.1, B1 = 0$

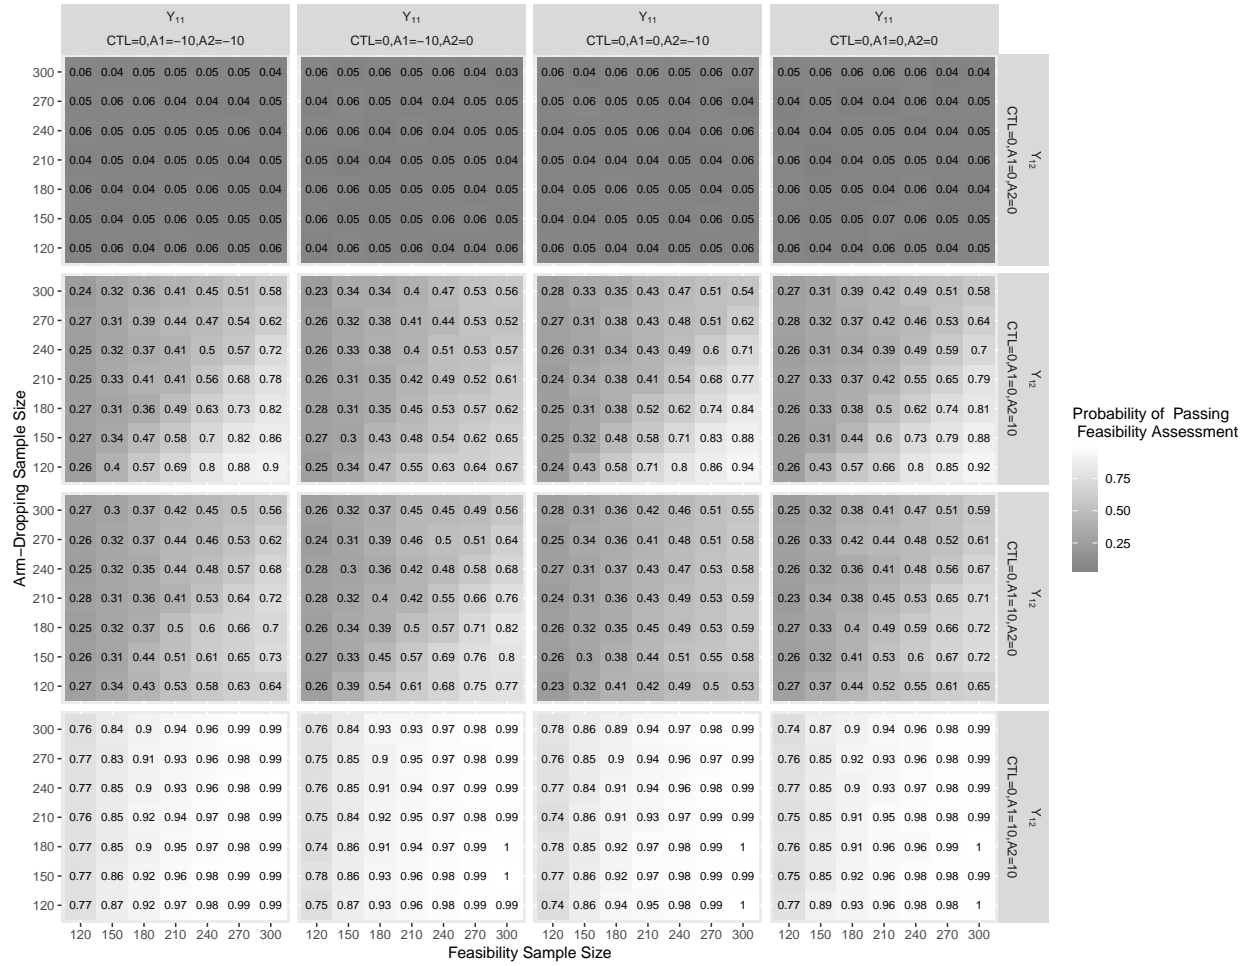

Probability Passing Feasibility Assessment  
by Timing of Feasibility and Arm-Dropping Analyses  
Treatment Effect:  $A1 = 0.1, A2 = 0, B1 = -0.1$

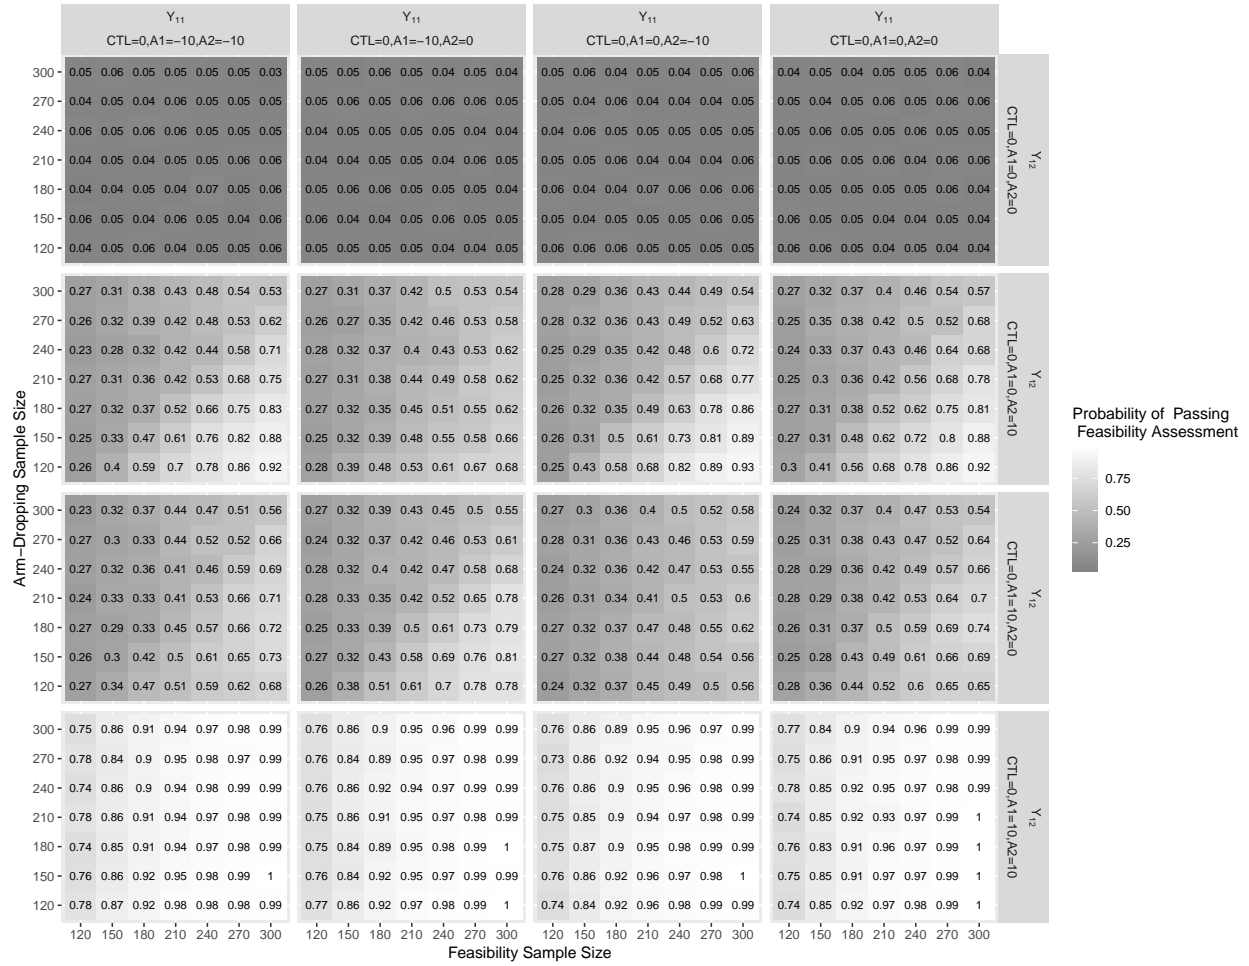

Probability Passing Feasibility Assessment  
by Timing of Feasibility and Arm-Dropping Analyses  
Treatment Effect:  $A1 = 0.1, A2 = 0, B1 = 0$

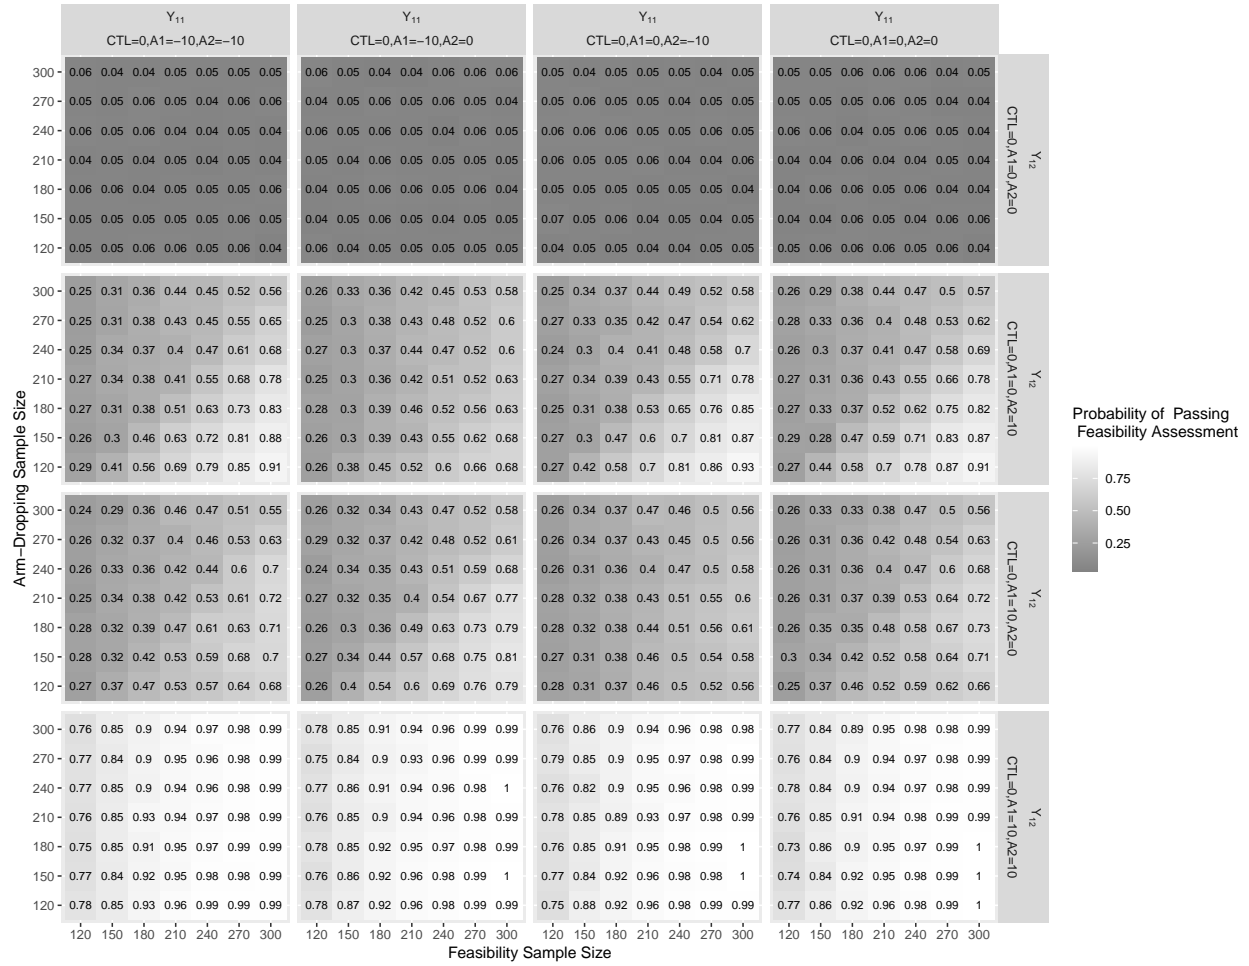

Probability Passing Feasibility Assessment  
by Timing of Feasibility and Arm-Dropping Analyses  
Treatment Effect:  $A1 = 0.1$ ,  $A2 = 0.1$ ,  $B1 = -0.1$

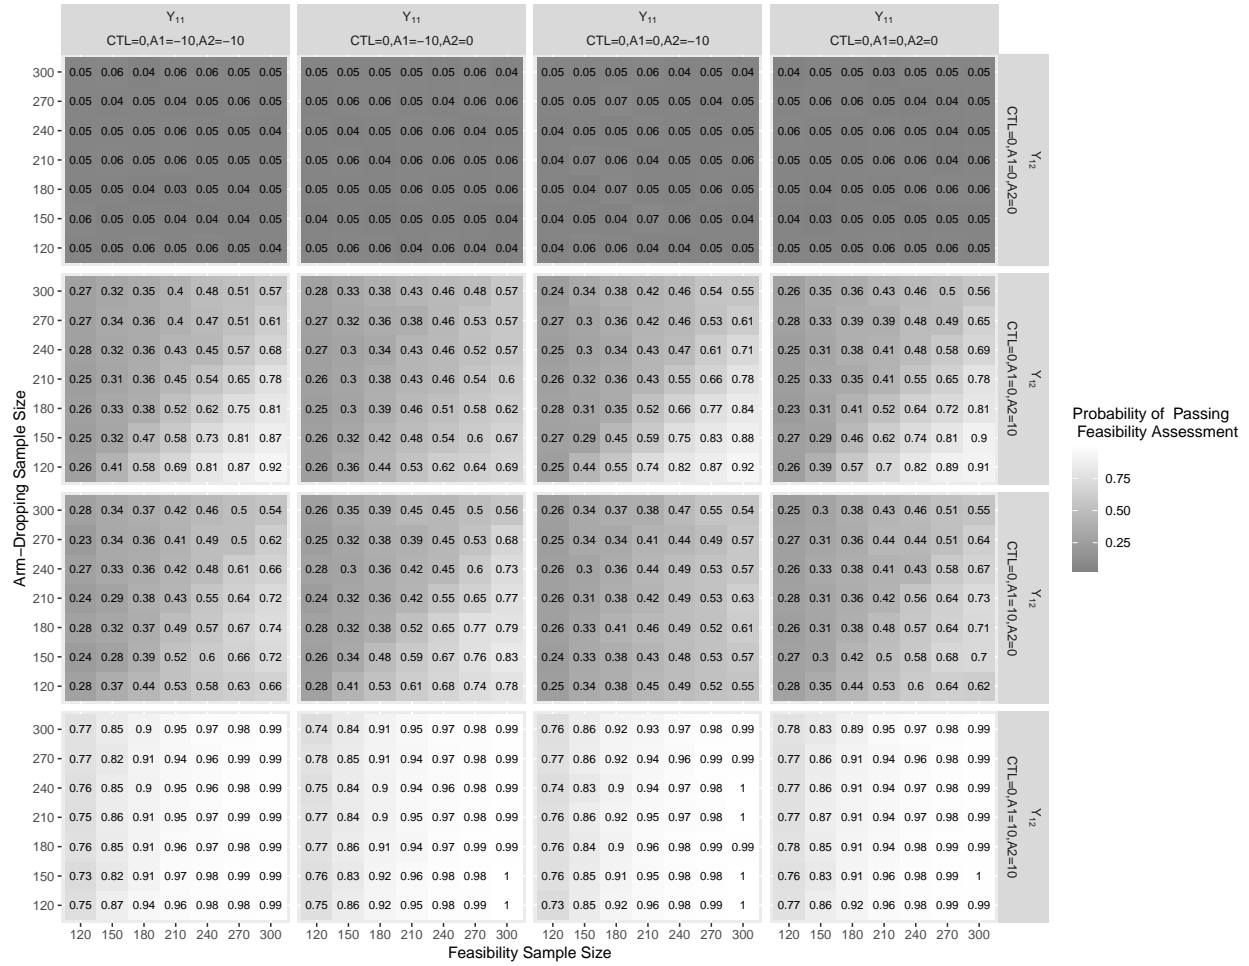

Probability Passing Feasibility Assessment  
by Timing of Feasibility and Arm-Dropping Analyses  
Treatment Effect:  $A1 = 0.1, A2 = 0.1, B1 = 0$

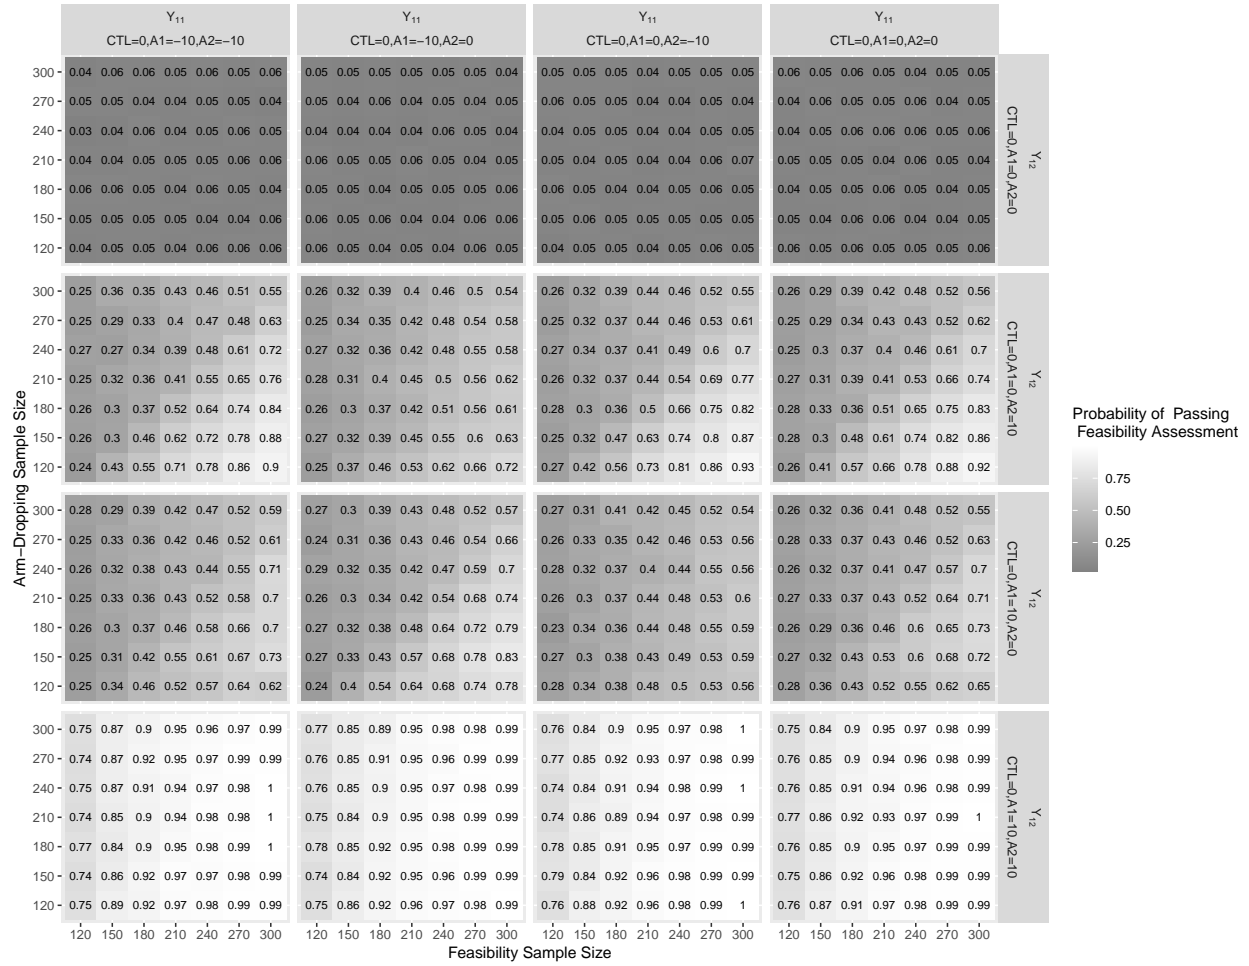

Supplement: Supplementary file 1 [file AppendixA.pdf]
