# Supplementary material for: Design Considerations for Factorial Adaptive Multi-Arm Multi-Stage (FAST) Clinical Trials
Source: arXiv:2310.12830 source file (2023-10-19)
Supplement: Supplementary file 2 [file AppendixB.pdf]

## Appendix B: Tables

Table 1: Simulation Results for the scenario where for  $Y_{11}$ : CTL=0,A1=-10,A2=-10 and  $Y_{12}$ : CTL=0,A1=0,A2=0. Under this scenario, the correct arm to retain during the arm-dropping analysis is A2. The feasibility and arm dropping analysis occurs once 300 and 150 outcomes have been obtained, respectively.

| Condition                     | Arm Dropping Analysis |       |       |                     | Feasibility Analysis | Phase III Analysis |       |       |       |       |       |       |       |       | Overall Operating Characteristics |  |
|-------------------------------|-----------------------|-------|-------|---------------------|----------------------|--------------------|-------|-------|-------|-------|-------|-------|-------|-------|-----------------------------------|--|
| Treatment Effect              | A1                    | A2    | Both  | P(Correct Decision) | P(Continue)          | A2:A1:B1           | A2:A1 | A2:B1 | A1:B1 | A2    | A1    | B1    | None  | Power | Type I Error                      |  |
| A1 = 0, A2 = 0, B1 = 0        | 0.046                 | 0.953 | 0.001 | 0.953               | 0.058                | 0                  | 0     | 0.000 | 0.000 | 0.002 | 0.000 | 0.046 | 0.952 | NA    | 0.048                             |  |
| A1 = 0, A2 = 0, B1 = -0.1     | 0.040                 | 0.960 | 0.000 | 0.960               | 0.051                | 0                  | 0     | 0.002 | 0.000 | 0.000 | 0.000 | 0.876 | 0.122 | 0.876 | 0.002                             |  |
| A1 = 0.1, A2 = 0, B1 = 0      | 0.045                 | 0.955 | 0.000 | 0.955               | 0.054                | 0                  | 0     | 0.000 | 0.000 | 0.003 | 0.004 | 0.059 | 0.934 | 0.004 | 0.062                             |  |
| A1 = 0.1, A2 = 0, B1 = -0.1   | 0.047                 | 0.953 | 0.000 | 0.953               | 0.057                | 0                  | 0     | 0.002 | 0.000 | 0.000 | 0.001 | 0.877 | 0.120 | 0.878 | 0.002                             |  |
| A1 = 0, A2 = 0.1, B1 = 0      | 0.048                 | 0.952 | 0.000 | 0.952               | 0.054                | 0                  | 0     | 0.002 | 0.000 | 0.031 | 0.000 | 0.053 | 0.914 | 0.031 | 0.055                             |  |
| A1 = 0, A2 = 0.1, B1 = -0.1   | 0.044                 | 0.955 | 0.001 | 0.955               | 0.054                | 0                  | 0     | 0.038 | 0.000 | 0.002 | 0.000 | 0.844 | 0.116 | 0.884 | 0.000                             |  |
| A1 = 0.1, A2 = 0.1, B1 = 0    | 0.046                 | 0.954 | 0.000 | 0.954               | 0.056                | 0                  | 0     | 0.001 | 0.001 | 0.040 | 0.001 | 0.049 | 0.908 | 0.041 | 0.051                             |  |
| A1 = 0.1, A2 = 0.1, B1 = -0.1 | 0.047                 | 0.952 | 0.001 | 0.952               | 0.049                | 0                  | 0     | 0.039 | 0.002 | 0.004 | 0.001 | 0.834 | 0.120 | 0.880 | NA                                |  |

Table 2: Simulation Results for the scenario where for  $Y_{11}$ : CTL=0,A1=-10,A2=0 and  $Y_{12}$ : CTL=0,A1=0,A2=0. Under this scenario, the correct arm to retain during the arm-dropping analysis is A1. The feasibility and arm dropping analysis occurs once 300 and 150 outcomes have been obtained, respectively.

| Condition                     | Arm Dropping Analysis |       |       |                     | Feasibility Analysis | Phase III Analysis |       |       |       |       |       |       |       |       | Overall Operating Characteristics |  |
|-------------------------------|-----------------------|-------|-------|---------------------|----------------------|--------------------|-------|-------|-------|-------|-------|-------|-------|-------|-----------------------------------|--|
| Treatment Effect              | A1                    | A2    | Both  | P(Correct Decision) | P(Continue)          | A2:A1:B1           | A2:A1 | A2:B1 | A1:B1 | A2    | A1    | B1    | None  | Power | Type I Error                      |  |
| A1 = 0, A2 = 0, B1 = 0        | 0.537                 | 0.450 | 0.013 | 0.537               | 0.049                | 0                  | 0     | 0.000 | 0.000 | 0.000 | 0.002 | 0.044 | 0.954 | NA    | 0.046                             |  |
| A1 = 0, A2 = 0, B1 = -0.1     | 0.550                 | 0.438 | 0.012 | 0.550               | 0.038                | 0                  | 0     | 0.001 | 0.001 | 0.001 | 0.000 | 0.903 | 0.094 | 0.903 | 0.003                             |  |
| A1 = 0.1, A2 = 0, B1 = 0      | 0.591                 | 0.393 | 0.016 | 0.591               | 0.046                | 0                  | 0     | 0.000 | 0.000 | 0.002 | 0.015 | 0.043 | 0.940 | 0.015 | 0.045                             |  |
| A1 = 0.1, A2 = 0, B1 = -0.1   | 0.567                 | 0.421 | 0.012 | 0.567               | 0.049                | 0                  | 0     | 0.002 | 0.022 | 0.000 | 0.001 | 0.865 | 0.110 | 0.888 | 0.002                             |  |
| A1 = 0, A2 = 0.1, B1 = 0      | 0.563                 | 0.421 | 0.016 | 0.563               | 0.049                | 0                  | 0     | 0.000 | 0.000 | 0.012 | 0.000 | 0.046 | 0.942 | 0.012 | 0.046                             |  |
| A1 = 0, A2 = 0.1, B1 = -0.1   | 0.601                 | 0.381 | 0.018 | 0.601               | 0.052                | 0                  | 0     | 0.015 | 0.002 | 0.003 | 0.000 | 0.865 | 0.115 | 0.883 | 0.002                             |  |
| A1 = 0.1, A2 = 0.1, B1 = 0    | 0.546                 | 0.440 | 0.014 | 0.546               | 0.057                | 0                  | 0     | 0.001 | 0.001 | 0.021 | 0.021 | 0.054 | 0.902 | 0.042 | 0.056                             |  |
| A1 = 0.1, A2 = 0.1, B1 = -0.1 | 0.522                 | 0.463 | 0.015 | 0.522               | 0.037                | 0                  | 0     | 0.015 | 0.013 | 0.002 | 0.002 | 0.865 | 0.103 | 0.897 | NA                                |  |

Table 3: Simulation Results for the scenario where for  $Y_{11}$ : CTL=0,A1=0,A2=-10 and  $Y_{12}$ : CTL=0,A1=0,A2=0. Under this scenario, the correct arm to retain during the arm-dropping analysis is A2. The feasibility and arm dropping analysis occurs once 300 and 150 outcomes have been obtained, respectively.

| Condition                     | Arm Dropping Analysis |       |       |                     | Feasibility Analysis | Phase III Analysis |       |       |       |       |       |       |       | Overall Operating Characteristics |              |
|-------------------------------|-----------------------|-------|-------|---------------------|----------------------|--------------------|-------|-------|-------|-------|-------|-------|-------|-----------------------------------|--------------|
| Treatment Effect              | A1                    | A2    | Both  | P(Correct Decision) | P(Continue)          | A2:A1:B1           | A2:A1 | A2:B1 | A1:B1 | A2    | A1    | B1    | None  | Power                             | Type I Error |
| A1 = 0, A2 = 0, B1 = 0        | 0.009                 | 0.979 | 0.012 | 0.979               | 0.046                | 0.000              | 0.000 | 0.000 | 0.000 | 0.001 | 0.000 | 0.038 | 0.961 | NA                                | 0.039        |
| A1 = 0, A2 = 0, B1 = -0.1     | 0.008                 | 0.985 | 0.007 | 0.985               | 0.041                | 0.000              | 0.000 | 0.001 | 0.000 | 0.000 | 0.000 | 0.899 | 0.100 | 0.899                             | 0.001        |
| A1 = 0.1, A2 = 0, B1 = 0      | 0.014                 | 0.978 | 0.008 | 0.978               | 0.051                | 0.000              | 0.000 | 0.000 | 0.000 | 0.000 | 0.000 | 0.045 | 0.955 | 0.000                             | 0.045        |
| A1 = 0.1, A2 = 0, B1 = -0.1   | 0.015                 | 0.970 | 0.015 | 0.970               | 0.050                | 0.000              | 0.000 | 0.002 | 0.002 | 0.000 | 0.001 | 0.888 | 0.107 | 0.891                             | 0.002        |
| A1 = 0, A2 = 0.1, B1 = 0      | 0.011                 | 0.971 | 0.018 | 0.971               | 0.049                | 0.000              | 0.000 | 0.002 | 0.000 | 0.033 | 0.000 | 0.040 | 0.925 | 0.033                             | 0.042        |
| A1 = 0, A2 = 0.1, B1 = -0.1   | 0.011                 | 0.976 | 0.013 | 0.976               | 0.053                | 0.000              | 0.000 | 0.036 | 0.000 | 0.008 | 0.000 | 0.849 | 0.107 | 0.893                             | 0.000        |
| A1 = 0.1, A2 = 0.1, B1 = 0    | 0.010                 | 0.974 | 0.016 | 0.974               | 0.046                | 0.000              | 0.001 | 0.001 | 0.000 | 0.030 | 0.001 | 0.051 | 0.916 | 0.032                             | 0.052        |
| A1 = 0.1, A2 = 0.1, B1 = -0.1 | 0.012                 | 0.970 | 0.018 | 0.970               | 0.045                | 0.001              | 0.000 | 0.031 | 0.000 | 0.006 | 0.000 | 0.826 | 0.136 | 0.864                             | NA           |

Table 4: Simulation Results for the scenario where for  $Y_{11}$ : CTL=0,A1=0,A2=0 and  $Y_{12}$ : CTL=0,A1=0,A2=0. Under this scenario, the correct arm to retain during the arm-dropping analysis is A2. The feasibility and arm dropping analysis occurs once 300 and 150 outcomes have been obtained, respectively.

| Condition                     | Arm Dropping Analysis |       |       |                     | Feasibility Analysis | Phase III Analysis |       |       |       |       |       |       |       |       | Overall Operating Characteristics |  |
|-------------------------------|-----------------------|-------|-------|---------------------|----------------------|--------------------|-------|-------|-------|-------|-------|-------|-------|-------|-----------------------------------|--|
| Treatment Effect              | A1                    | A2    | Both  | P(Correct Decision) | P(Continue)          | A2:A1:B1           | A2:A1 | A2:B1 | A1:B1 | A2    | A1    | B1    | None  | Power | Type I Error                      |  |
| A1 = 0, A2 = 0, B1 = 0        | 0.048                 | 0.952 | 0.000 | 0.952               | 0.043                | 0                  | 0     | 0.000 | 0.000 | 0.002 | 0.000 | 0.053 | 0.945 | NA    | 0.055                             |  |
| A1 = 0, A2 = 0, B1 = -0.1     | 0.043                 | 0.955 | 0.002 | 0.955               | 0.060                | 0                  | 0     | 0.000 | 0.000 | 0.000 | 0.000 | 0.890 | 0.110 | 0.890 | 0.000                             |  |
| A1 = 0.1, A2 = 0, B1 = 0      | 0.051                 | 0.947 | 0.002 | 0.947               | 0.055                | 0                  | 0     | 0.000 | 0.000 | 0.000 | 0.000 | 0.045 | 0.955 | 0.000 | 0.045                             |  |
| A1 = 0.1, A2 = 0, B1 = -0.1   | 0.052                 | 0.948 | 0.000 | 0.948               | 0.043                | 0                  | 0     | 0.006 | 0.002 | 0.000 | 0.000 | 0.875 | 0.117 | 0.877 | 0.006                             |  |
| A1 = 0, A2 = 0.1, B1 = 0      | 0.037                 | 0.963 | 0.000 | 0.963               | 0.051                | 0                  | 0     | 0.000 | 0.000 | 0.033 | 0.000 | 0.056 | 0.911 | 0.033 | 0.056                             |  |
| A1 = 0, A2 = 0.1, B1 = -0.1   | 0.043                 | 0.955 | 0.002 | 0.955               | 0.051                | 0                  | 0     | 0.032 | 0.000 | 0.005 | 0.000 | 0.840 | 0.123 | 0.877 | 0.000                             |  |
| A1 = 0.1, A2 = 0.1, B1 = 0    | 0.049                 | 0.949 | 0.002 | 0.949               | 0.054                | 0                  | 0     | 0.005 | 0.000 | 0.037 | 0.000 | 0.059 | 0.899 | 0.037 | 0.064                             |  |
| A1 = 0.1, A2 = 0.1, B1 = -0.1 | 0.048                 | 0.949 | 0.003 | 0.949               | 0.053                | 0                  | 0     | 0.043 | 0.001 | 0.004 | 0.001 | 0.835 | 0.116 | 0.884 | NA                                |  |

Table 5: Simulation Results for the scenario where for  $Y_{11}$ : CTL=0,A1=-10,A2=-10 and  $Y_{12}$ : CTL=0,A1=0,A2=10. Under this scenario, the correct arm to retain during the arm-dropping analysis is A2. The feasibility and arm dropping analysis occurs once 300 and 150 outcomes have been obtained, respectively.

| Condition                     | Arm Dropping Analysis |       |       |                     | Feasibility Analysis | Phase III Analysis |       |       |       |       |       |       |       |       | Overall Operating Characteristics |  |
|-------------------------------|-----------------------|-------|-------|---------------------|----------------------|--------------------|-------|-------|-------|-------|-------|-------|-------|-------|-----------------------------------|--|
| Treatment Effect              | A1                    | A2    | Both  | P(Correct Decision) | P(Continue)          | A2:A1:B1           | A2:A1 | A2:B1 | A1:B1 | A2    | A1    | B1    | None  | Power | Type I Error                      |  |
| A1 = 0, A2 = 0, B1 = 0        | 0.007                 | 0.970 | 0.023 | 0.970               | 0.888                | 0.000              | 0.000 | 0.003 | 0.000 | 0.020 | 0.001 | 0.021 | 0.955 | NA    | 0.045                             |  |
| A1 = 0, A2 = 0, B1 = -0.1     | 0.006                 | 0.981 | 0.013 | 0.981               | 0.883                | 0.000              | 0.000 | 0.042 | 0.000 | 0.003 | 0.000 | 0.788 | 0.167 | 0.788 | 0.045                             |  |
| A1 = 0.1, A2 = 0, B1 = 0      | 0.007                 | 0.978 | 0.015 | 0.978               | 0.878                | 0.000              | 0.001 | 0.002 | 0.000 | 0.022 | 0.008 | 0.021 | 0.946 | 0.008 | 0.046                             |  |
| A1 = 0.1, A2 = 0, B1 = -0.1   | 0.008                 | 0.966 | 0.026 | 0.966               | 0.876                | 0.000              | 0.001 | 0.041 | 0.005 | 0.004 | 0.008 | 0.768 | 0.173 | 0.781 | 0.046                             |  |
| A1 = 0, A2 = 0.1, B1 = 0      | 0.004                 | 0.978 | 0.018 | 0.978               | 0.855                | 0.000              | 0.000 | 0.034 | 0.001 | 0.544 | 0.000 | 0.013 | 0.408 | 0.544 | 0.048                             |  |
| A1 = 0, A2 = 0.1, B1 = -0.1   | 0.006                 | 0.976 | 0.018 | 0.976               | 0.880                | 0.000              | 0.000 | 0.611 | 0.000 | 0.086 | 0.000 | 0.256 | 0.047 | 0.953 | 0.000                             |  |
| A1 = 0.1, A2 = 0.1, B1 = 0    | 0.005                 | 0.979 | 0.016 | 0.979               | 0.880                | 0.001              | 0.004 | 0.045 | 0.000 | 0.639 | 0.002 | 0.017 | 0.292 | 0.645 | 0.063                             |  |
| A1 = 0.1, A2 = 0.1, B1 = -0.1 | 0.009                 | 0.970 | 0.021 | 0.970               | 0.874                | 0.007              | 0.000 | 0.648 | 0.002 | 0.089 | 0.000 | 0.221 | 0.033 | 0.967 | NA                                |  |

Table 6: Simulation Results for the scenario where for  $Y_{11}$ : CTL=0,A1=-10,A2=0 and  $Y_{12}$ : CTL=0,A1=0,A2=10. Under this scenario, the correct arm to retain during the arm-dropping analysis is Both. The feasibility and arm dropping analysis occurs once 300 and 150 outcomes have been obtained, respectively.

| Condition                     | Arm Dropping Analysis |       |       |                     | Feasibility Analysis | Phase III Analysis |       |       |       |       |       |       |       |       | Overall Operating Characteristics |  |
|-------------------------------|-----------------------|-------|-------|---------------------|----------------------|--------------------|-------|-------|-------|-------|-------|-------|-------|-------|-----------------------------------|--|
| Treatment Effect              | A1                    | A2    | Both  | P(Correct Decision) | P(Continue)          | A2:A1:B1           | A2:A1 | A2:B1 | A1:B1 | A2    | A1    | B1    | None  | Power | Type I Error                      |  |
| A1 = 0, A2 = 0, B1 = 0        | 0.137                 | 0.433 | 0.430 | 0.430               | 0.656                | 0.000              | 0.001 | 0.000 | 0.000 | 0.008 | 0.000 | 0.027 | 0.964 | NA    | 0.036                             |  |
| A1 = 0, A2 = 0, B1 = -0.1     | 0.157                 | 0.420 | 0.423 | 0.423               | 0.638                | 0.000              | 0.000 | 0.021 | 0.006 | 0.001 | 0.003 | 0.819 | 0.150 | 0.819 | 0.031                             |  |
| A1 = 0.1, A2 = 0, B1 = 0      | 0.122                 | 0.442 | 0.436 | 0.436               | 0.677                | 0.002              | 0.003 | 0.002 | 0.004 | 0.010 | 0.147 | 0.029 | 0.803 | 0.147 | 0.050                             |  |
| A1 = 0.1, A2 = 0, B1 = -0.1   | 0.171                 | 0.427 | 0.402 | 0.402               | 0.655                | 0.005              | 0.001 | 0.015 | 0.152 | 0.004 | 0.044 | 0.658 | 0.121 | 0.854 | 0.025                             |  |
| A1 = 0, A2 = 0.1, B1 = 0      | 0.149                 | 0.404 | 0.447 | 0.447               | 0.654                | 0.000              | 0.001 | 0.015 | 0.001 | 0.380 | 0.002 | 0.025 | 0.576 | 0.380 | 0.044                             |  |
| A1 = 0, A2 = 0.1, B1 = -0.1   | 0.158                 | 0.436 | 0.406 | 0.406               | 0.649                | 0.005              | 0.000 | 0.389 | 0.005 | 0.068 | 0.001 | 0.463 | 0.069 | 0.920 | 0.011                             |  |
| A1 = 0.1, A2 = 0.1, B1 = 0    | 0.170                 | 0.406 | 0.424 | 0.424               | 0.626                | 0.010              | 0.083 | 0.006 | 0.005 | 0.289 | 0.047 | 0.026 | 0.534 | 0.419 | 0.047                             |  |
| A1 = 0.1, A2 = 0.1, B1 = -0.1 | 0.134                 | 0.458 | 0.408 | 0.408               | 0.667                | 0.121              | 0.026 | 0.336 | 0.039 | 0.038 | 0.004 | 0.373 | 0.063 | 0.937 | NA                                |  |

Table 7: Simulation Results for the scenario where for  $Y_{11}$ : CTL=0,A1=0,A2=-10 and  $Y_{12}$ : CTL=0,A1=0,A2=10. Under this scenario, the correct arm to retain during the arm-dropping analysis is A2. The feasibility and arm dropping analysis occurs once 300 and 150 outcomes have been obtained, respectively.

| Condition                     | Arm Dropping Analysis |    |      |                     | Feasibility Analysis | Phase III Analysis |       |       |       |       |    |       |       | Overall Operating Characteristics |              |
|-------------------------------|-----------------------|----|------|---------------------|----------------------|--------------------|-------|-------|-------|-------|----|-------|-------|-----------------------------------|--------------|
| Treatment Effect              | A1                    | A2 | Both | P(Correct Decision) | P(Continue)          | A2:A1:B1           | A2:A1 | A2:B1 | A1:B1 | A2    | A1 | B1    | None  | Power                             | Type I Error |
| A1 = 0, A2 = 0, B1 = 0        | 0                     | 1  | 0    | 1                   | 0.874                | 0                  | 0     | 0.004 | 0     | 0.020 | 0  | 0.022 | 0.954 | NA                                | 0.046        |
| A1 = 0, A2 = 0, B1 = -0.1     | 0                     | 1  | 0    | 1                   | 0.878                | 0                  | 0     | 0.037 | 0     | 0.003 | 0  | 0.806 | 0.154 | 0.806                             | 0.040        |
| A1 = 0.1, A2 = 0, B1 = 0      | 0                     | 1  | 0    | 1                   | 0.873                | 0                  | 0     | 0.001 | 0     | 0.032 | 0  | 0.025 | 0.942 | 0.000                             | 0.058        |
| A1 = 0.1, A2 = 0, B1 = -0.1   | 0                     | 1  | 0    | 1                   | 0.892                | 0                  | 0     | 0.059 | 0     | 0.000 | 0  | 0.793 | 0.148 | 0.793                             | 0.059        |
| A1 = 0, A2 = 0.1, B1 = 0      | 0                     | 1  | 0    | 1                   | 0.884                | 0                  | 0     | 0.030 | 0     | 0.558 | 0  | 0.017 | 0.395 | 0.558                             | 0.047        |
| A1 = 0, A2 = 0.1, B1 = -0.1   | 0                     | 1  | 0    | 1                   | 0.879                | 0                  | 0     | 0.597 | 0     | 0.093 | 0  | 0.262 | 0.048 | 0.952                             | 0.000        |
| A1 = 0.1, A2 = 0.1, B1 = 0    | 0                     | 1  | 0    | 1                   | 0.873                | 0                  | 0     | 0.041 | 0     | 0.622 | 0  | 0.012 | 0.325 | 0.622                             | 0.053        |
| A1 = 0.1, A2 = 0.1, B1 = -0.1 | 0                     | 1  | 0    | 1                   | 0.880                | 0                  | 0     | 0.676 | 0     | 0.094 | 0  | 0.196 | 0.034 | 0.966                             | NA           |

Table 8: Simulation Results for the scenario where for  $Y_{11}$ : CTL=0,A1=0,A2=0 and  $Y_{12}$ : CTL=0,A1=0,A2=10. Under this scenario, the correct arm to retain during the arm-dropping analysis is A2. The feasibility and arm dropping analysis occurs once 300 and 150 outcomes have been obtained, respectively.

| Condition                     | Arm Dropping Analysis |       |       |                     | Feasibility Analysis | Phase III Analysis |       |       |       |       |       |       |       |       | Overall Operating Characteristics |  |
|-------------------------------|-----------------------|-------|-------|---------------------|----------------------|--------------------|-------|-------|-------|-------|-------|-------|-------|-------|-----------------------------------|--|
| Treatment Effect              | A1                    | A2    | Both  | P(Correct Decision) | P(Continue)          | A2:A1:B1           | A2:A1 | A2:B1 | A1:B1 | A2    | A1    | B1    | None  | Power | Type I Error                      |  |
| A1 = 0, A2 = 0, B1 = 0        | 0.004                 | 0.972 | 0.024 | 0.972               | 0.880                | 0.000              | 0.000 | 0.001 | 0.000 | 0.020 | 0.000 | 0.023 | 0.956 | NA    | 0.044                             |  |
| A1 = 0, A2 = 0, B1 = -0.1     | 0.008                 | 0.974 | 0.018 | 0.974               | 0.873                | 0.000              | 0.000 | 0.039 | 0.000 | 0.002 | 0.000 | 0.792 | 0.167 | 0.792 | 0.041                             |  |
| A1 = 0.1, A2 = 0, B1 = 0      | 0.007                 | 0.977 | 0.016 | 0.977               | 0.871                | 0.000              | 0.000 | 0.004 | 0.000 | 0.022 | 0.009 | 0.020 | 0.945 | 0.009 | 0.046                             |  |
| A1 = 0.1, A2 = 0, B1 = -0.1   | 0.007                 | 0.982 | 0.011 | 0.982               | 0.882                | 0.001              | 0.000 | 0.040 | 0.005 | 0.001 | 0.002 | 0.800 | 0.151 | 0.807 | 0.042                             |  |
| A1 = 0, A2 = 0.1, B1 = 0      | 0.005                 | 0.981 | 0.014 | 0.981               | 0.876                | 0.000              | 0.000 | 0.028 | 0.000 | 0.557 | 0.000 | 0.018 | 0.397 | 0.557 | 0.046                             |  |
| A1 = 0, A2 = 0.1, B1 = -0.1   | 0.009                 | 0.977 | 0.014 | 0.977               | 0.870                | 0.000              | 0.000 | 0.631 | 0.000 | 0.075 | 0.000 | 0.265 | 0.029 | 0.971 | 0.000                             |  |
| A1 = 0.1, A2 = 0.1, B1 = 0    | 0.006                 | 0.973 | 0.021 | 0.973               | 0.863                | 0.000              | 0.004 | 0.035 | 0.000 | 0.601 | 0.001 | 0.010 | 0.349 | 0.606 | 0.045                             |  |
| A1 = 0.1, A2 = 0.1, B1 = -0.1 | 0.002                 | 0.985 | 0.013 | 0.985               | 0.895                | 0.003              | 0.002 | 0.699 | 0.000 | 0.084 | 0.000 | 0.179 | 0.033 | 0.967 | NA                                |  |

Table 9: Simulation Results for the scenario where for  $Y_{11}$ : CTL=0,A1=-10,A2=-10 and  $Y_{12}$ : CTL=0,A1=10,A2=0. Under this scenario, the correct arm to retain during the arm-dropping analysis is A1. The feasibility and arm dropping analysis occurs once 300 and 150 outcomes have been obtained, respectively.

| Condition                     | Arm Dropping Analysis |       |       |                     | Feasibility Analysis | Phase III Analysis |       |       |       |       |       |       |       |       | Overall Operating Characteristics |  |
|-------------------------------|-----------------------|-------|-------|---------------------|----------------------|--------------------|-------|-------|-------|-------|-------|-------|-------|-------|-----------------------------------|--|
| Treatment Effect              | A1                    | A2    | Both  | P(Correct Decision) | P(Continue)          | A2:A1:B1           | A2:A1 | A2:B1 | A1:B1 | A2    | A1    | B1    | None  | Power | Type I Error                      |  |
| A1 = 0, A2 = 0, B1 = 0        | 0.736                 | 0.250 | 0.014 | 0.736               | 0.718                | 0.000              | 0.000 | 0.000 | 0.000 | 0.002 | 0.018 | 0.026 | 0.954 | NA    | 0.046                             |  |
| A1 = 0, A2 = 0, B1 = -0.1     | 0.721                 | 0.265 | 0.014 | 0.721               | 0.696                | 0.000              | 0.000 | 0.002 | 0.022 | 0.000 | 0.004 | 0.828 | 0.144 | 0.828 | 0.028                             |  |
| A1 = 0.1, A2 = 0, B1 = 0      | 0.728                 | 0.250 | 0.022 | 0.728               | 0.701                | 0.000              | 0.001 | 0.000 | 0.013 | 0.003 | 0.411 | 0.019 | 0.553 | 0.411 | 0.036                             |  |
| A1 = 0.1, A2 = 0, B1 = -0.1   | 0.724                 | 0.259 | 0.017 | 0.724               | 0.729                | 0.000              | 0.000 | 0.003 | 0.449 | 0.001 | 0.067 | 0.406 | 0.074 | 0.922 | 0.004                             |  |
| A1 = 0, A2 = 0.1, B1 = 0      | 0.740                 | 0.251 | 0.009 | 0.740               | 0.726                | 0.000              | 0.000 | 0.005 | 0.003 | 0.032 | 0.025 | 0.029 | 0.906 | 0.032 | 0.062                             |  |
| A1 = 0, A2 = 0.1, B1 = -0.1   | 0.749                 | 0.236 | 0.015 | 0.749               | 0.725                | 0.000              | 0.000 | 0.047 | 0.032 | 0.008 | 0.007 | 0.757 | 0.149 | 0.812 | 0.039                             |  |
| A1 = 0.1, A2 = 0.1, B1 = 0    | 0.719                 | 0.268 | 0.013 | 0.719               | 0.731                | 0.000              | 0.002 | 0.003 | 0.016 | 0.057 | 0.489 | 0.018 | 0.415 | 0.548 | 0.037                             |  |
| A1 = 0.1, A2 = 0.1, B1 = -0.1 | 0.733                 | 0.254 | 0.013 | 0.733               | 0.719                | 0.004              | 0.000 | 0.051 | 0.504 | 0.005 | 0.061 | 0.327 | 0.048 | 0.952 | NA                                |  |

Table 10: Simulation Results for the scenario where for  $Y_{11}$ : CTL=0,A1=-10,A2=0 and  $Y_{12}$ : CTL=0,A1=10,A2=0. Under this scenario, the correct arm to retain during the arm-dropping analysis is A1. The feasibility and arm dropping analysis occurs once 300 and 150 outcomes have been obtained, respectively.

| Condition                     | Arm Dropping Analysis |       |      |                     | Feasibility Analysis | Phase III Analysis |       |       |       |       |       |       |       |       | Overall Operating Characteristics |  |
|-------------------------------|-----------------------|-------|------|---------------------|----------------------|--------------------|-------|-------|-------|-------|-------|-------|-------|-------|-----------------------------------|--|
| Treatment Effect              | A1                    | A2    | Both | P(Correct Decision) | P(Continue)          | A2:A1:B1           | A2:A1 | A2:B1 | A1:B1 | A2    | A1    | B1    | None  | Power | Type I Error                      |  |
| A1 = 0, A2 = 0, B1 = 0        | 0.897                 | 0.103 | 0    | 0.897               | 0.810                | 0                  | 0     | 0.000 | 0.001 | 0.000 | 0.009 | 0.020 | 0.970 | NA    | 0.030                             |  |
| A1 = 0, A2 = 0, B1 = -0.1     | 0.895                 | 0.105 | 0    | 0.895               | 0.831                | 0                  | 0     | 0.001 | 0.032 | 0.000 | 0.003 | 0.807 | 0.157 | 0.807 | 0.036                             |  |
| A1 = 0.1, A2 = 0, B1 = 0      | 0.887                 | 0.113 | 0    | 0.887               | 0.811                | 0                  | 0     | 0.000 | 0.028 | 0.001 | 0.498 | 0.017 | 0.456 | 0.498 | 0.046                             |  |
| A1 = 0.1, A2 = 0, B1 = -0.1   | 0.878                 | 0.122 | 0    | 0.878               | 0.811                | 0                  | 0     | 0.000 | 0.550 | 0.000 | 0.067 | 0.332 | 0.051 | 0.949 | 0.000                             |  |
| A1 = 0, A2 = 0.1, B1 = 0      | 0.871                 | 0.129 | 0    | 0.871               | 0.798                | 0                  | 0     | 0.004 | 0.003 | 0.017 | 0.035 | 0.029 | 0.912 | 0.017 | 0.071                             |  |
| A1 = 0, A2 = 0.1, B1 = -0.1   | 0.891                 | 0.109 | 0    | 0.891               | 0.819                | 0                  | 0     | 0.019 | 0.045 | 0.006 | 0.001 | 0.773 | 0.156 | 0.798 | 0.046                             |  |
| A1 = 0.1, A2 = 0.1, B1 = 0    | 0.903                 | 0.097 | 0    | 0.903               | 0.834                | 0                  | 0     | 0.001 | 0.039 | 0.027 | 0.592 | 0.012 | 0.329 | 0.619 | 0.052                             |  |
| A1 = 0.1, A2 = 0.1, B1 = -0.1 | 0.894                 | 0.106 | 0    | 0.894               | 0.833                | 0                  | 0     | 0.017 | 0.615 | 0.006 | 0.092 | 0.229 | 0.041 | 0.959 | NA                                |  |

Table 11: Simulation Results for the scenario where for  $Y_{11}$ : CTL=0,A1=0,A2=-10 and  $Y_{12}$ : CTL=0,A1=10,A2=0. Under this scenario, the correct arm to retain during the arm-dropping analysis is Both. The feasibility and arm dropping analysis occurs once 300 and 150 outcomes have been obtained, respectively.

| Condition                     | Arm Dropping Analysis |       |       |                     | Feasibility Analysis | Phase III Analysis |       |       |       |       |       |       |       |       | Overall Operating Characteristics |  |
|-------------------------------|-----------------------|-------|-------|---------------------|----------------------|--------------------|-------|-------|-------|-------|-------|-------|-------|-------|-----------------------------------|--|
| Treatment Effect              | A1                    | A2    | Both  | P(Correct Decision) | P(Continue)          | A2:A1:B1           | A2:A1 | A2:B1 | A1:B1 | A2    | A1    | B1    | None  | Power | Type I Error                      |  |
| A1 = 0, A2 = 0, B1 = 0        | 0.290                 | 0.256 | 0.454 | 0.454               | 0.576                | 0.000              | 0.001 | 0.000 | 0.000 | 0.001 | 0.014 | 0.039 | 0.945 | NA    | 0.055                             |  |
| A1 = 0, A2 = 0, B1 = -0.1     | 0.317                 | 0.292 | 0.391 | 0.391               | 0.551                | 0.000              | 0.000 | 0.002 | 0.021 | 0.004 | 0.002 | 0.822 | 0.149 | 0.822 | 0.029                             |  |
| A1 = 0.1, A2 = 0, B1 = 0      | 0.324                 | 0.276 | 0.400 | 0.400               | 0.584                | 0.000              | 0.001 | 0.000 | 0.013 | 0.002 | 0.289 | 0.025 | 0.670 | 0.289 | 0.041                             |  |
| A1 = 0.1, A2 = 0, B1 = -0.1   | 0.313                 | 0.285 | 0.402 | 0.402               | 0.555                | 0.006              | 0.000 | 0.007 | 0.305 | 0.000 | 0.049 | 0.544 | 0.089 | 0.898 | 0.013                             |  |
| A1 = 0, A2 = 0.1, B1 = 0      | 0.322                 | 0.259 | 0.419 | 0.419               | 0.581                | 0.000              | 0.004 | 0.007 | 0.001 | 0.158 | 0.011 | 0.026 | 0.793 | 0.158 | 0.049                             |  |
| A1 = 0, A2 = 0.1, B1 = -0.1   | 0.298                 | 0.292 | 0.410 | 0.410               | 0.568                | 0.007              | 0.001 | 0.172 | 0.013 | 0.026 | 0.004 | 0.652 | 0.125 | 0.850 | 0.025                             |  |
| A1 = 0.1, A2 = 0.1, B1 = 0    | 0.317                 | 0.256 | 0.427 | 0.427               | 0.589                | 0.003              | 0.105 | 0.003 | 0.015 | 0.071 | 0.234 | 0.023 | 0.546 | 0.410 | 0.044                             |  |
| A1 = 0.1, A2 = 0.1, B1 = -0.1 | 0.310                 | 0.256 | 0.434 | 0.434               | 0.573                | 0.123              | 0.020 | 0.059 | 0.223 | 0.012 | 0.029 | 0.464 | 0.070 | 0.930 | NA                                |  |

Table 12: Simulation Results for the scenario where for  $Y_{11}$ : CTL=0,A1=0,A2=0 and  $Y_{12}$ : CTL=0,A1=10,A2=0. Under this scenario, the correct arm to retain during the arm-dropping analysis is A1. The feasibility and arm dropping analysis occurs once 300 and 150 outcomes have been obtained, respectively.

| Condition                     | Arm Dropping Analysis |       |       |                     | Feasibility Analysis | Phase III Analysis |       |       |       |       |       |       |       |       | Overall Operating Characteristics |  |
|-------------------------------|-----------------------|-------|-------|---------------------|----------------------|--------------------|-------|-------|-------|-------|-------|-------|-------|-------|-----------------------------------|--|
| Treatment Effect              | A1                    | A2    | Both  | P(Correct Decision) | P(Continue)          | A2:A1:B1           | A2:A1 | A2:B1 | A1:B1 | A2    | A1    | B1    | None  | Power | Type I Error                      |  |
| A1 = 0, A2 = 0, B1 = 0        | 0.735                 | 0.247 | 0.018 | 0.735               | 0.707                | 0.000              | 0.000 | 0.000 | 0.002 | 0.001 | 0.013 | 0.022 | 0.962 | NA    | 0.038                             |  |
| A1 = 0, A2 = 0, B1 = -0.1     | 0.715                 | 0.262 | 0.023 | 0.715               | 0.726                | 0.000              | 0.000 | 0.006 | 0.026 | 0.000 | 0.001 | 0.806 | 0.161 | 0.806 | 0.033                             |  |
| A1 = 0.1, A2 = 0, B1 = 0      | 0.722                 | 0.261 | 0.017 | 0.722               | 0.708                | 0.000              | 0.000 | 0.000 | 0.017 | 0.002 | 0.427 | 0.026 | 0.528 | 0.427 | 0.045                             |  |
| A1 = 0.1, A2 = 0, B1 = -0.1   | 0.721                 | 0.265 | 0.014 | 0.721               | 0.687                | 0.000              | 0.000 | 0.006 | 0.445 | 0.000 | 0.060 | 0.420 | 0.069 | 0.925 | 0.006                             |  |
| A1 = 0, A2 = 0.1, B1 = 0      | 0.737                 | 0.242 | 0.021 | 0.737               | 0.724                | 0.000              | 0.000 | 0.001 | 0.001 | 0.045 | 0.020 | 0.024 | 0.909 | 0.045 | 0.046                             |  |
| A1 = 0, A2 = 0.1, B1 = -0.1   | 0.735                 | 0.253 | 0.012 | 0.735               | 0.735                | 0.001              | 0.000 | 0.051 | 0.043 | 0.008 | 0.005 | 0.759 | 0.133 | 0.818 | 0.049                             |  |
| A1 = 0.1, A2 = 0.1, B1 = 0    | 0.717                 | 0.264 | 0.019 | 0.717               | 0.716                | 0.000              | 0.006 | 0.003 | 0.027 | 0.052 | 0.459 | 0.021 | 0.432 | 0.517 | 0.051                             |  |
| A1 = 0.1, A2 = 0.1, B1 = -0.1 | 0.695                 | 0.290 | 0.015 | 0.695               | 0.704                | 0.005              | 0.001 | 0.053 | 0.479 | 0.012 | 0.066 | 0.341 | 0.043 | 0.957 | NA                                |  |

Table 13: Simulation Results for the scenario where for  $Y_{11}$ : CTL=0,A1=-10,A2=-10 and  $Y_{12}$ : CTL=0,A1=10,A2=10. Under this scenario, the correct arm to retain during the arm-dropping analysis is A2. The feasibility and arm dropping analysis occurs once 300 and 150 outcomes have been obtained, respectively.

| Condition                     | Arm Dropping Analysis |       |       |                     | Feasibility Analysis | Phase III Analysis |       |       |       |       |       |       |       |       | Overall Operating Characteristics |  |
|-------------------------------|-----------------------|-------|-------|---------------------|----------------------|--------------------|-------|-------|-------|-------|-------|-------|-------|-------|-----------------------------------|--|
| Treatment Effect              | A1                    | A2    | Both  | P(Correct Decision) | P(Continue)          | A2:A1:B1           | A2:A1 | A2:B1 | A1:B1 | A2    | A1    | B1    | None  | Power | Type I Error                      |  |
| A1 = 0, A2 = 0, B1 = 0        | 0.038                 | 0.962 | 0.000 | 0.962               | 0.993                | 0                  | 0     | 0.003 | 0.000 | 0.025 | 0.002 | 0.024 | 0.946 | NA    | 0.054                             |  |
| A1 = 0, A2 = 0, B1 = -0.1     | 0.060                 | 0.938 | 0.002 | 0.938               | 0.992                | 0                  | 0     | 0.042 | 0.002 | 0.003 | 0.000 | 0.764 | 0.189 | 0.764 | 0.047                             |  |
| A1 = 0.1, A2 = 0, B1 = 0      | 0.036                 | 0.963 | 0.001 | 0.963               | 0.989                | 0                  | 0     | 0.002 | 0.000 | 0.034 | 0.023 | 0.022 | 0.919 | 0.023 | 0.058                             |  |
| A1 = 0.1, A2 = 0, B1 = -0.1   | 0.052                 | 0.948 | 0.000 | 0.948               | 0.997                | 0                  | 0     | 0.050 | 0.033 | 0.004 | 0.007 | 0.742 | 0.164 | 0.782 | 0.054                             |  |
| A1 = 0, A2 = 0.1, B1 = 0      | 0.054                 | 0.944 | 0.002 | 0.944               | 0.993                | 0                  | 0     | 0.027 | 0.001 | 0.608 | 0.003 | 0.005 | 0.356 | 0.608 | 0.036                             |  |
| A1 = 0, A2 = 0.1, B1 = -0.1   | 0.055                 | 0.943 | 0.002 | 0.943               | 0.995                | 0                  | 0     | 0.664 | 0.003 | 0.099 | 0.000 | 0.189 | 0.045 | 0.952 | 0.003                             |  |
| A1 = 0.1, A2 = 0.1, B1 = 0    | 0.044                 | 0.956 | 0.000 | 0.956               | 0.990                | 0                  | 0     | 0.037 | 0.001 | 0.689 | 0.033 | 0.011 | 0.229 | 0.722 | 0.049                             |  |
| A1 = 0.1, A2 = 0.1, B1 = -0.1 | 0.047                 | 0.953 | 0.000 | 0.953               | 0.994                | 0                  | 0     | 0.731 | 0.034 | 0.107 | 0.004 | 0.096 | 0.028 | 0.972 | NA                                |  |

Table 14: Simulation Results for the scenario where for  $Y_{11}$ : CTL=0,A1=-10,A2=0 and  $Y_{12}$ : CTL=0,A1=10,A2=10. Under this scenario, the correct arm to retain during the arm-dropping analysis is A1. The feasibility and arm dropping analysis occurs once 300 and 150 outcomes have been obtained, respectively.

| Condition                     | Arm Dropping Analysis |       |       |                     | Feasibility Analysis | Phase III Analysis |       |       |       |       |       |       |       |       | Overall Operating Characteristics |  |
|-------------------------------|-----------------------|-------|-------|---------------------|----------------------|--------------------|-------|-------|-------|-------|-------|-------|-------|-------|-----------------------------------|--|
| Treatment Effect              | A1                    | A2    | Both  | P(Correct Decision) | P(Continue)          | A2:A1:B1           | A2:A1 | A2:B1 | A1:B1 | A2    | A1    | B1    | None  | Power | Type I Error                      |  |
| A1 = 0, A2 = 0, B1 = 0        | 0.554                 | 0.436 | 0.010 | 0.554               | 0.989                | 0.000              | 0.000 | 0.000 | 0.001 | 0.012 | 0.017 | 0.026 | 0.944 | NA    | 0.056                             |  |
| A1 = 0, A2 = 0, B1 = -0.1     | 0.540                 | 0.444 | 0.016 | 0.540               | 0.993                | 0.000              | 0.000 | 0.025 | 0.023 | 0.003 | 0.002 | 0.777 | 0.170 | 0.777 | 0.053                             |  |
| A1 = 0.1, A2 = 0, B1 = 0      | 0.560                 | 0.424 | 0.016 | 0.560               | 0.996                | 0.000              | 0.000 | 0.001 | 0.035 | 0.013 | 0.364 | 0.012 | 0.575 | 0.364 | 0.061                             |  |
| A1 = 0.1, A2 = 0, B1 = -0.1   | 0.559                 | 0.428 | 0.013 | 0.559               | 0.992                | 0.000              | 0.000 | 0.023 | 0.400 | 0.003 | 0.059 | 0.438 | 0.077 | 0.897 | 0.026                             |  |
| A1 = 0, A2 = 0.1, B1 = 0      | 0.559                 | 0.415 | 0.026 | 0.559               | 0.997                | 0.000              | 0.001 | 0.015 | 0.000 | 0.271 | 0.017 | 0.014 | 0.682 | 0.271 | 0.047                             |  |
| A1 = 0, A2 = 0.1, B1 = -0.1   | 0.560                 | 0.422 | 0.018 | 0.560               | 0.989                | 0.000              | 0.000 | 0.312 | 0.024 | 0.034 | 0.003 | 0.514 | 0.113 | 0.860 | 0.027                             |  |
| A1 = 0.1, A2 = 0.1, B1 = 0    | 0.563                 | 0.422 | 0.015 | 0.563               | 0.990                | 0.000              | 0.003 | 0.018 | 0.034 | 0.308 | 0.414 | 0.008 | 0.215 | 0.725 | 0.060                             |  |
| A1 = 0.1, A2 = 0.1, B1 = -0.1 | 0.581                 | 0.406 | 0.013 | 0.581               | 0.996                | 0.007              | 0.001 | 0.303 | 0.457 | 0.040 | 0.061 | 0.111 | 0.020 | 0.980 | NA                                |  |

Table 15: Simulation Results for the scenario where for  $Y_{11}$ : CTL=0,A1=0,A2=-10 and  $Y_{12}$ : CTL=0,A1=10,A2=10. Under this scenario, the correct arm to retain during the arm-dropping analysis is A2. The feasibility and arm dropping analysis occurs once 300 and 150 outcomes have been obtained, respectively.

| Condition                     | Arm Dropping Analysis |       |       |                     | Feasibility Analysis | Phase III Analysis |       |       |       |       |       |       |       | Overall Operating Characteristics |              |
|-------------------------------|-----------------------|-------|-------|---------------------|----------------------|--------------------|-------|-------|-------|-------|-------|-------|-------|-----------------------------------|--------------|
| Treatment Effect              | A1                    | A2    | Both  | P(Correct Decision) | P(Continue)          | A2:A1:B1           | A2:A1 | A2:B1 | A1:B1 | A2    | A1    | B1    | None  | Power                             | Type I Error |
| A1 = 0, A2 = 0, B1 = 0        | 0.006                 | 0.977 | 0.017 | 0.977               | 0.993                | 0.000              | 0.000 | 0.006 | 0.000 | 0.025 | 0.001 | 0.012 | 0.956 | NA                                | 0.044        |
| A1 = 0, A2 = 0, B1 = -0.1     | 0.008                 | 0.981 | 0.011 | 0.981               | 0.994                | 0.001              | 0.000 | 0.042 | 0.000 | 0.006 | 0.001 | 0.784 | 0.166 | 0.784                             | 0.050        |
| A1 = 0.1, A2 = 0, B1 = 0      | 0.008                 | 0.970 | 0.022 | 0.970               | 0.995                | 0.000              | 0.002 | 0.006 | 0.001 | 0.034 | 0.015 | 0.017 | 0.925 | 0.015                             | 0.060        |
| A1 = 0.1, A2 = 0, B1 = -0.1   | 0.009                 | 0.980 | 0.011 | 0.980               | 0.995                | 0.001              | 0.000 | 0.045 | 0.008 | 0.006 | 0.002 | 0.777 | 0.161 | 0.787                             | 0.052        |
| A1 = 0, A2 = 0.1, B1 = 0      | 0.015                 | 0.971 | 0.014 | 0.971               | 0.994                | 0.000              | 0.000 | 0.040 | 0.000 | 0.640 | 0.001 | 0.008 | 0.311 | 0.640                             | 0.049        |
| A1 = 0, A2 = 0.1, B1 = -0.1   | 0.007                 | 0.985 | 0.008 | 0.985               | 0.997                | 0.000              | 0.000 | 0.705 | 0.000 | 0.086 | 0.000 | 0.168 | 0.041 | 0.959                             | 0.000        |
| A1 = 0.1, A2 = 0.1, B1 = 0    | 0.006                 | 0.971 | 0.023 | 0.971               | 0.994                | 0.000              | 0.009 | 0.035 | 0.001 | 0.729 | 0.007 | 0.010 | 0.209 | 0.745                             | 0.046        |
| A1 = 0.1, A2 = 0.1, B1 = -0.1 | 0.011                 | 0.979 | 0.010 | 0.979               | 0.999                | 0.005              | 0.000 | 0.759 | 0.008 | 0.107 | 0.002 | 0.098 | 0.021 | 0.979                             | NA           |

Table 16: Simulation Results for the scenario where for  $Y_{11}$ : CTL=0,A1=0,A2=0 and  $Y_{12}$ : CTL=0,A1=10,A2=10. Under this scenario, the correct arm to retain during the arm-dropping analysis is A2. The feasibility and arm dropping analysis occurs once 300 and 150 outcomes have been obtained, respectively.

| Condition                     | Arm Dropping Analysis |       |       |                     | Feasibility Analysis | Phase III Analysis |       |       |       |       |       |       |       | Overall Operating Characteristics |              |
|-------------------------------|-----------------------|-------|-------|---------------------|----------------------|--------------------|-------|-------|-------|-------|-------|-------|-------|-----------------------------------|--------------|
| Treatment Effect              | A1                    | A2    | Both  | P(Correct Decision) | P(Continue)          | A2:A1:B1           | A2:A1 | A2:B1 | A1:B1 | A2    | A1    | B1    | None  | Power                             | Type I Error |
| A1 = 0, A2 = 0, B1 = 0        | 0.047                 | 0.952 | 0.001 | 0.952               | 0.993                | 0                  | 0.000 | 0.001 | 0.000 | 0.018 | 0.001 | 0.024 | 0.956 | NA                                | 0.044        |
| A1 = 0, A2 = 0, B1 = -0.1     | 0.043                 | 0.954 | 0.003 | 0.954               | 0.995                | 0                  | 0.000 | 0.036 | 0.004 | 0.005 | 0.000 | 0.797 | 0.158 | 0.797                             | 0.045        |
| A1 = 0.1, A2 = 0, B1 = 0      | 0.035                 | 0.964 | 0.001 | 0.964               | 0.997                | 0                  | 0.000 | 0.003 | 0.001 | 0.025 | 0.018 | 0.022 | 0.931 | 0.018                             | 0.051        |
| A1 = 0.1, A2 = 0, B1 = -0.1   | 0.055                 | 0.944 | 0.001 | 0.944               | 0.995                | 0                  | 0.000 | 0.054 | 0.041 | 0.001 | 0.005 | 0.708 | 0.191 | 0.754                             | 0.055        |
| A1 = 0, A2 = 0.1, B1 = 0      | 0.052                 | 0.946 | 0.002 | 0.946               | 0.990                | 0                  | 0.000 | 0.033 | 0.000 | 0.610 | 0.001 | 0.015 | 0.341 | 0.610                             | 0.049        |
| A1 = 0, A2 = 0.1, B1 = -0.1   | 0.051                 | 0.949 | 0.000 | 0.949               | 0.990                | 0                  | 0.000 | 0.685 | 0.002 | 0.077 | 0.001 | 0.202 | 0.033 | 0.964                             | 0.003        |
| A1 = 0.1, A2 = 0.1, B1 = 0    | 0.058                 | 0.938 | 0.004 | 0.938               | 0.991                | 0                  | 0.002 | 0.043 | 0.002 | 0.640 | 0.039 | 0.011 | 0.263 | 0.681                             | 0.056        |
| A1 = 0.1, A2 = 0.1, B1 = -0.1 | 0.053                 | 0.947 | 0.000 | 0.947               | 0.995                | 0                  | 0.000 | 0.729 | 0.043 | 0.105 | 0.006 | 0.099 | 0.018 | 0.982                             | NA           |
